# Supplementary material for: Efficient Treatment of Relativistic Effects with Periodic Density Functional Methods: Energies, Gradients, and Stress Tensors
Source: arXiv:2305.03817 source file (2024-03-16)
Supplement: Supplementary file 1 [file supplemental-material_V12.pdf]

# Supplemental Material: Efficient Treatment of Relativistic Effects with Periodic Density Functional Methods: Energies, Gradients, and Stress Tensors

Yannick J. Franzke,[1,2] Werner M. Schosser,[3] and Fabian Pauly[3,*]

[1]*Fachbereich Chemie, Philipps-Universität Marburg, Hans-Meerwein-Str. 4, 35032 Marburg, Germany*

[2]*Otto Schott Institute of Materials Research, Friedrich Schiller University Jena, Löbdergraben 32, 07743 Jena, Germany*[†]

[3]*Institute of Physics and Center for Advanced Analytics and Predictive Sciences, University of Augsburg, Universitätsstr. 1, 86159 Augsburg, Germany*[†]

(Dated: March 16, 2024)

**CONTENTS**

I. Basis Set Study of Silver Halide Crystals with Non-Relaxed Structure 3

II. Density Functional Approximation Study of Silver Halide Crystals with Relaxed Structures: Scalar-Relativistic and Spin–Orbit Results 6

III. Indium(I,III)-Telluride Two-Dimensional Honeycomb System 9

IV. One-Dimensional Platinum Chains 11

V. Structures 21

A. SCF Computation Times 21

B. Ionization Energies of Zero-Dimensional Heavy $p$-Block Atoms 22

C. Band Structures of Three-Dimensional Gold and Lead Crystals 23

D. Band Gaps of Three-Dimensional Silver Halide Crystals 24

E. Indium(I,III)-Telluride Two-Dimensional Honeycomb System 43

F. One-Dimensional Platinum Chains 44

References 49

* fabian.pauly@uni-a.de

† Y.J.F. and W.M.S. contributed equally to this work

## I. BASIS SET STUDY OF SILVER HALIDE CRYSTALS WITH NON-RELAXED STRUCTURE

TABLE I. Band gaps (in eV) of three-dimensional AgCl (lattice constant $a = 5.612\,\text{Å}$, rocksalt structure [1]) at high symmetry points of the FBZ. The local spin density approximation (LSDA) is represented by the S-VWN (V) functional [2, 3], whereas PBE [4] and PBEsol [5] serve as examples for generalized gradient approximations (GGAs). Meta-GGAs are included through the TPSS [6], revTPSS [7, 8], Tao–Mo [9], PKZB [10], and r$^2$SCAN [11, 12] approximations. Note that we use Libxc [13–15] for the PBEsol, revTPSS, Tao–Mo, PKZB, and r$^2$SCAN functionals. The dhf-SVP and dhf-TZVP basis sets are employed [16].

| | One-Component | | | | Two-Component | | | |
|---|---|---|---|---|---|---|---|---|
| dhf-SVP | L–L | Γ–Γ | X–X | L–Γ | L–L | Γ–Γ | X–X | L–Γ |
| S-VWN (V) | 4.30 | 2.83 | 3.90 | 0.59 | 4.25 | 2.70 | 3.73 | 0.54 |
| PBE | 4.62 | 3.11 | 4.16 | 0.91 | 4.57 | 2.94 | 3.99 | 0.86 |
| PBEsol | 4.38 | 2.95 | 4.02 | 0.72 | 4.33 | 2.78 | 3.85 | 0.67 |
| TPSS | 4.65 | 3.16 | 4.29 | 1.03 | 4.60 | 3.00 | 4.12 | 0.98 |
| revTPSS | 4.52 | 3.10 | 4.27 | 0.96 | 4.46 | 2.93 | 4.10 | 0.90 |
| Tao–Mo | 4.38 | 3.12 | 4.36 | 1.03 | 4.33 | 2.96 | 4.20 | 0.97 |
| PKZB | 4.61 | 3.29 | 4.42 | 1.22 | 4.56 | 3.14 | 4.27 | 1.17 |
| r$^2$SCAN | 5.11 | 3.64 | 4.71 | 1.47 | 5.06 | 3.47 | 4.55 | 1.41 |
| dhf-TZVP | L–L | Γ–Γ | X–X | L–Γ | L–L | Γ–Γ | X–X | L–Γ |
| S-VWN (V) | 4.09 | 2.77 | 3.79 | 0.54 | 4.04 | 2.68 | 3.62 | 0.49 |
| PBE | 4.37 | 3.07 | 4.03 | 0.85 | 4.32 | 2.90 | 3.86 | 0.80 |
| PBEsol | 4.16 | 2.91 | 3.90 | 0.66 | 4.11 | 2.75 | 3.72 | 0.61 |
| TPSS | 4.39 | 3.11 | 4.15 | 0.94 | 4.33 | 2.94 | 3.99 | 0.89 |
| revTPSS | 4.28 | 3.04 | 4.14 | 0.87 | 4.23 | 2.88 | 3.97 | 0.82 |
| Tao–Mo | 4.21 | 3.07 | 4.23 | 0.95 | 4.15 | 2.92 | 4.07 | 0.90 |
| PKZB | 4.44 | 3.26 | 4.29 | 1.17 | 4.39 | 3.11 | 4.14 | 1.11 |
| r$^2$SCAN | 4.87 | 3.59 | 4.57 | 1.38 | 4.82 | 3.42 | 4.41 | 1.33 |

TABLE II. Band gaps (in eV) of three-dimensional AgBr (lattice constant $a = 5.843\,\text{Å}$, rocksalt structure [1]) at high symmetry points of the FBZ. The local spin density approximation (LSDA) is represented by the S-VWN (V) functional [2, 3], whereas PBE [4] and PBEsol [5] serve as examples for generalized gradient approximations (GGAs). Meta-GGAs are included through the TPSS [6], revTPSS [7, 8], Tao–Mo [9], PKZB [10], and r$^2$SCAN [11, 12] approximations. Note that we use Libxc [13–15] for the PBEsol, revTPSS, Tao–Mo, PKZB, and r$^2$SCAN functionals. The dhf-SVP and dhf-TZVP basis sets are employed [16].

| | One-Component | | | | Two-Component | | | |
|---|---|---|---|---|---|---|---|---|
| dhf-SVP | L–L | Γ–Γ | X–X | L–Γ | L–L | Γ–Γ | X–X | L–Γ |
| S-VWN (V) | 3.81 | 2.34 | 3.47 | 0.54 | 3.76 | 2.33 | 3.31 | 0.50 |
| PBE | 4.07 | 2.64 | 3.70 | 0.86 | 4.02 | 2.64 | 3.54 | 0.82 |
| PBEsol | 3.87 | 2.49 | 3.57 | 0.68 | 3.82 | 2.48 | 3.41 | 0.64 |
| TPSS | 4.08 | 2.85 | 3.82 | 1.00 | 4.04 | 2.85 | 3.67 | 0.95 |
| revTPSS | 4.01 | 2.87 | 3.80 | 0.99 | 3.96 | 2.86 | 3.65 | 0.94 |
| Tao–Mo | 3.97 | 2.94 | 3.91 | 1.11 | 3.92 | 2.93 | 3.76 | 1.06 |
| PKZB | 4.14 | 3.03 | 3.96 | 1.23 | 4.09 | 3.03 | 3.81 | 1.19 |
| r$^2$SCAN | 4.59 | 3.30 | 4.24 | 1.46 | 4.54 | 3.30 | 4.09 | 1.41 |
| dhf-TZVP | L–L | Γ–Γ | X–X | L–Γ | L–L | Γ–Γ | X–X | L–Γ |
| S-VWN (V) | 3.71 | 2.32 | 3.42 | 0.51 | 3.67 | 2.31 | 3.26 | 0.47 |
| PBE | 3.96 | 2.62 | 3.63 | 0.81 | 3.91 | 2.62 | 3.48 | 0.77 |
| PBEsol | 3.77 | 2.47 | 3.51 | 0.64 | 3.72 | 2.46 | 3.35 | 0.60 |
| TPSS | 3.99 | 2.83 | 3.75 | 0.95 | 3.94 | 2.82 | 3.60 | 0.90 |
| revTPSS | 3.92 | 2.83 | 3.73 | 0.92 | 3.87 | 2.82 | 3.58 | 0.88 |
| Tao–Mo | 3.89 | 2.89 | 3.83 | 1.04 | 3.84 | 2.88 | 3.68 | 0.99 |
| PKZB | 4.07 | 3.00 | 3.89 | 1.18 | 4.02 | 2.99 | 3.74 | 1.13 |
| r$^2$SCAN | 4.48 | 3.27 | 4.16 | 1.40 | 4.43 | 3.27 | 4.01 | 1.36 |

TABLE III. Band gaps (in eV) of three-dimensional AgI (lattice constant $a = 6.169$ Å, rocksalt structure [1]) at high symmetry points of the FBZ. The local spin density approximation (LSDA) is represented by the S-VWN (V) functional, [2, 3] whereas PBE [4] and PBEsol [5] serve as examples for generalized gradient approximations (GGAs). Meta-GGAs are included through the TPSS [6], revTPSS [7, 8], Tao–Mo [9], PKZB [10], and r$^2$SCAN [11, 12] approximations. Note that we use Libxc [13–15] for the PBEsol, revTPSS, Tao–Mo, PKZB, and r$^2$SCAN functionals. The dhf-SVP and dhf-TZVP basis sets are employed [16].

| | One-Component | | | | Two-Component | | | |
|---|---|---|---|---|---|---|---|---|
| dhf-SVP | L–L | Γ–Γ | X–X | L–Γ | L–L | Γ–Γ | X–X | L–Γ |
| S-VWN (V) | 3.29 | 1.88 | 2.76 | 0.40 | 3.04 | 1.53 | 2.47 | 0.15 |
| PBE | 3.49 | 2.16 | 2.98 | 0.65 | 3.25 | 1.82 | 2.69 | 0.41 |
| PBEsol | 3.32 | 2.02 | 2.89 | 0.53 | 3.08 | 1.67 | 2.60 | 0.29 |
| TPSS | 3.51 | 2.37 | 3.21 | 0.84 | 3.27 | 2.02 | 2.92 | 0.60 |
| revTPSS | 3.46 | 2.39 | 3.24 | 0.84 | 3.23 | 2.05 | 2.95 | 0.61 |
| Tao–Mo | 3.46 | 2.51 | 3.30 | 0.97 | 3.23 | 2.17 | 3.02 | 0.74 |
| PKZB | 3.60 | 2.54 | 3.30 | 1.01 | 3.37 | 2.20 | 3.01 | 0.78 |
| r$^2$SCAN | 4.02 | 2.83 | 3.52 | 1.16 | 3.79 | 2.48 | 3.23 | 0.92 |
| dhf-TZVP | L–L | Γ–Γ | X–X | L–Γ | L–L | Γ–Γ | X–X | L–Γ |
| S-VWN (V) | 3.22 | 1.86 | 2.75 | 0.38 | 2.96 | 1.51 | 2.46 | 0.12 |
| PBE | 3.39 | 2.14 | 2.95 | 0.60 | 3.15 | 1.79 | 2.66 | 0.36 |
| PBEsol | 3.24 | 2.00 | 2.87 | 0.49 | 2.99 | 1.65 | 2.58 | 0.24 |
| TPSS | 3.43 | 2.34 | 3.18 | 0.79 | 3.18 | 2.00 | 2.89 | 0.55 |
| revTPSS | 3.37 | 2.36 | 3.20 | 0.78 | 3.13 | 2.01 | 2.91 | 0.55 |
| Tao–Mo | 3.37 | 2.47 | 3.26 | 0.91 | 3.13 | 2.12 | 2.97 | 0.68 |
| PKZB | 3.50 | 2.50 | 3.26 | 0.95 | 3.26 | 2.15 | 2.97 | 0.71 |
| r$^2$SCAN | 3.92 | 2.80 | 3.49 | 1.10 | 3.68 | 2.46 | 3.20 | 0.86 |

## II. DENSITY FUNCTIONAL APPROXIMATION STUDY OF SILVER HALIDE CRYSTALS WITH RELAXED STRUCTURES: SCALAR-RELATIVISTIC AND SPIN–ORBIT RESULTS

TABLE IV. Band gaps (in eV) at high symmetry points of the FBZ and optimized lattice constant $a$ (in Å) of three-dimensional AgCl (rocksalt structure). The local spin density approximation (LSDA) is represented by the S-VWN (V) functional [2, 3], whereas PBE [4] and PBEsol [5] serve as examples for generalized gradient approximations (GGAs). Meta-GGAs are included through the TPSS [6], revTPSS [7, 8], Tao–Mo [9], PKZB [10], and r$^2$SCAN [11, 12] approximations. Note that we use Libxc [13–15] for the PBEsol, revTPSS, Tao–Mo, PKZB, and r$^2$SCAN functionals. The dhf-SVP basis set is employed [16]. The D3 correction with Becke–Johnson (BJ) damping [17, 18] is applied if stated explicitly. The experimental result for $a$ is 5.550 Å [19].

| | | One-Component | | | | | Two-Component | | | | |
|---|---|---|---|---|---|---|---|---|---|---|---|
| Functional | Dispersion | $a$ | L–L | Γ–Γ | X–X | L–Γ | $a$ | L–L | Γ–Γ | X–X | L–Γ |
| S-VWN (V) | no D3 | 5.442 | 4.08 | 3.21 | 3.96 | 0.59 | 5.377 | 3.93 | 3.27 | 3.85 | 0.55 |
| PBE | no D3 | 5.627 | 4.64 | 3.08 | 4.16 | 0.92 | 5.624 | 4.58 | 2.91 | 3.99 | 0.86 |
| PBEsol | no D3 | 5.517 | 4.26 | 3.14 | 4.05 | 0.71 | 5.515 | 4.20 | 2.98 | 3.89 | 0.66 |
| TPSS | no D3 | 5.589 | 4.61 | 3.20 | 4.30 | 1.02 | 5.586 | 4.55 | 3.04 | 4.13 | 0.97 |
| revTPSS | no D3 | 5.562 | 4.44 | 3.18 | 4.29 | 0.94 | 5.561 | 4.38 | 3.02 | 4.13 | 0.89 |
| Tao–Mo | no D3 | 5.542 | 4.29 | 3.25 | 4.39 | 1.02 | 5.541 | 4.24 | 3.10 | 4.24 | 0.97 |
| PKZB | no D3 | 5.640 | 4.65 | 3.25 | 4.41 | 1.23 | 5.636 | 4.59 | 3.10 | 4.26 | 1.18 |
| r$^2$SCAN | no D3 | 5.578 | 5.07 | 3.71 | 4.72 | 1.47 | 5.576 | 5.02 | 3.55 | 4.56 | 1.41 |
| Functional | Dispersion | $a$ | L–L | Γ–Γ | X–X | L–Γ | $a$ | L–L | Γ–Γ | X–X | L–Γ |
| PBE | D3-BJ | 5.556 | 4.54 | 3.21 | 4.18 | 0.90 | 5.537 | 4.47 | 3.08 | 4.03 | 0.85 |
| PBEsol | D3-BJ | 5.428 | 4.12 | 3.36 | 4.08 | 0.71 | 5.426 | 4.07 | 3.20 | 3.93 | 0.66 |
| TPSS | D3-BJ | 5.500 | 4.46 | 3.37 | 4.33 | 1.00 | 5.498 | 4.40 | 3.21 | 4.18 | 0.94 |
| revTPSS | D3-BJ | 5.476 | 4.29 | 3.36 | 4.32 | 0.93 | 5.476 | 4.23 | 3.20 | 4.17 | 0.87 |
| Tao–Mo | D3-BJ | 5.513 | 4.26 | 3.32 | 4.40 | 1.02 | 5.511 | 4.20 | 3.17 | 4.25 | 0.97 |
| r$^2$SCAN | D3-BJ | 5.535 | 5.02 | 3.80 | 4.73 | 1.47 | 5.517 | 4.94 | 3.68 | 4.59 | 1.42 |

TABLE V. Band gaps (in eV) at high symmetry points of the FBZ and optimized lattice constant $a$ (in Å) of three-dimensional AgBr (rocksalt structure). The local spin density approximation (LSDA) is represented by the S-VWN (V) functional [2, 3], whereas PBE [4] and PBEsol [5] serve as examples for generalized gradient approximations (GGAs). Meta-GGAs are included through the TPSS [6], revTPSS [7, 8], Tao–Mo [9], PKZB [10], and r$^2$SCAN [11, 12] approximations. Note that we use Libxc [13–15] for the PBEsol, revTPSS, Tao–Mo, PKZB, and r$^2$SCAN functionals. The dhf-SVP basis set is employed [16]. The D3 correction with Becke–Johnson (BJ) damping [17, 18] is applied if stated explicitly. The experimental result for $a$ is 5.774 Å [20].

| | | One-Component | | | | | Two-Component | | | | |
|---|---|---|---|---|---|---|---|---|---|---|---|
| Functional | Dispersion | $a$ | L–L | Γ–Γ | X–X | L–Γ | $a$ | L–L | Γ–Γ | X–X | L–Γ |
| S-VWN (V) | no D3 | 5.609 | 3.47 | 2.82 | 3.52 | 0.58 | 5.604 | 3.42 | 2.82 | 3.39 | 0.54 |
| PBE | no D3 | 5.852 | 4.08 | 2.63 | 3.70 | 0.86 | 5.849 | 4.03 | 2.63 | 3.54 | 0.82 |
| PBEsol | no D3 | 5.695 | 3.66 | 2.77 | 3.59 | 0.70 | 5.692 | 3.60 | 2.77 | 3.45 | 0.65 |
| TPSS | no D3 | 5.815 | 4.04 | 2.90 | 3.83 | 1.00 | 5.812 | 3.99 | 2.90 | 3.68 | 0.95 |
| revTPSS | no D3 | 5.789 | 3.93 | 2.96 | 3.81 | 0.98 | 5.784 | 3.87 | 2.96 | 3.67 | 0.94 |
| Tao–Mo | no D3 | 5.773 | 3.88 | 3.07 | 3.92 | 1.12 | 5.738 | 3.78 | 3.14 | 3.79 | 1.08 |
| PKZB | no D3 | 5.867 | 4.17 | 2.99 | 3.96 | 1.24 | 5.868 | 4.13 | 2.99 | 3.81 | 1.19 |
| r$^2$SCAN | no D3 | 5.814 | 4.55 | 3.36 | 4.24 | 1.46 | 5.811 | 4.50 | 3.36 | 4.09 | 1.42 |
| Functional | Dispersion | $a$ | L–L | Γ–Γ | X–X | L–Γ | $a$ | L–L | Γ–Γ | X–X | L–Γ |
| PBE | D3-BJ | 5.750 | 3.94 | 2.82 | 3.72 | 0.87 | 5.747 | 3.89 | 2.82 | 3.57 | 0.83 |
| PBEsol | D3-BJ | 5.616 | 3.53 | 2.95 | 3.61 | 0.72 | 5.613 | 3.48 | 2.95 | 3.48 | 0.67 |
| TPSS | D3-BJ | 5.710 | 3.87 | 3.09 | 3.85 | 1.00 | 5.708 | 3.82 | 3.09 | 3.71 | 0.95 |
| revTPSS | D3-BJ | 5.692 | 3.77 | 3.15 | 3.83 | 0.99 | 5.690 | 3.72 | 3.14 | 3.70 | 0.94 |
| Tao–Mo | D3-BJ | 5.745 | 3.84 | 3.13 | 3.93 | 1.12 | 5.743 | 3.79 | 3.13 | 3.79 | 1.08 |
| r$^2$SCAN | D3-BJ | 5.774 | 4.50 | 3.45 | 4.25 | 1.47 | 5.772 | 4.45 | 3.44 | 4.10 | 1.42 |

TABLE VI. Band gaps (in eV) at high symmetry points of the FBZ and optimized lattice constant $a$ (in Å) of three-dimensional AgI (rocksalt structure). The local spin density approximation (LSDA) is represented by the S-VWN (V) functional [2, 3], whereas PBE [4] and PBEsol [5] serve as examples for generalized gradient approximations (GGAs). Meta-GGAs are included through the TPSS [6], revTPSS [7, 8], Tao–Mo [9], PKZB [10], and r$^2$SCAN [11, 12] approximations. Note that we use Libxc [13–15] for the PBEsol, revTPSS, Tao–Mo, PKZB, and r$^2$SCAN functionals. The dhf-SVP basis set is employed [16]. The D3 correction with Becke–Johnson (BJ) damping [17, 18] is applied if stated explicitly. The experimental result for $a$ is 6.067 Å [21].

| | | One-Component | | | | | Two-Component | | | | |
|---|---|---|---|---|---|---|---|---|---|---|---|
| Functional | Dispersion | $a$ | L–L | Γ–Γ | X–X | L–X | $a$ | L–L | Γ–Γ | X–X | L–X |
| S-VWN (V) | no D3 | 5.938 | 2.98 | 2.32 | 3.00 | 0.08 | 5.937 | 2.73 | 1.96 | 2.70 | −0.17 |
| PBE | no D3 | 6.189 | 3.52 | 2.13 | 2.96 | 0.68 | 6.187 | 3.27 | 1.79 | 2.67 | 0.44 |
| PBEsol | no D3 | 6.025 | 3.13 | 2.28 | 3.03 | 0.33 | 6.023 | 2.88 | 1.93 | 2.74 | 0.09 |
| TPSS | no D3 | 6.156 | 3.49 | 2.39 | 3.22 | 0.82 | 6.153 | 3.25 | 2.05 | 2.94 | 0.58 |
| revTPSS | no D3 | 6.118 | 3.39 | 2.48 | 3.28 | 0.77 | 6.116 | 3.15 | 2.13 | 3.00 | 0.54 |
| Tao–Mo | no D3 | 6.097 | 3.36 | 2.64 | 3.37 | 0.88 | 6.071 | 3.10 | 2.34 | 3.11 | 0.62 |
| PKZB | no D3 | 6.203 | 3.65 | 2.49 | 3.27 | 1.06 | 6.200 | 3.41 | 2.15 | 2.99 | 0.83 |
| r$^2$SCAN | no D3 | 6.161 | 4.01 | 2.84 | 3.52 | 1.15 | 6.159 | 3.78 | 2.50 | 3.24 | 0.91 |
| Functional | Dispersion | $a$ | L–L | Γ–Γ | X–X | L–X | $a$ | L–L | Γ–Γ | X–X | L–X |
| PBE | D3-BJ | 6.078 | 3.369 | 2.32 | 3.06 | 0.53 | 6.067 | 3.11 | 1.99 | 2.78 | 0.28 |
| PBEsol | D3-BJ | 5.930 | 2.986 | 2.48 | 3.13 | 0.19 | 5.927 | 2.74 | 2.12 | 2.84 | −0.06 |
| TPSS | D3-BJ | 5.983 | 3.227 | 2.71 | 3.37 | 0.58 | 5.982 | 2.99 | 2.35 | 3.10 | 0.34 |
| revTPSS | D3-BJ | 5.955 | 3.130 | 2.79 | 3.35 | 0.53 | 5.949 | 2.88 | 2.44 | 3.16 | 0.29 |
| Tao–Mo | D3-BJ | 6.078 | 3.339 | 2.67 | 3.39 | 0.85 | 6.068 | 3.10 | 2.35 | 3.11 | 0.61 |
| r$^2$SCAN | D3-BJ | 6.159 | 4.011 | 2.84 | 3.53 | 1.14 | 6.156 | 3.77 | 2.51 | 3.24 | 0.91 |

## III. INDIUM(I,III)-TELLURIDE TWO-DIMENSIONAL HONEYCOMB SYSTEM

Unit cell parameters and electronic band structures are calculated without the D3-BJ correction for comparison to the results in the main text. Additionally, the cell structure was optimized without taking spin–orbit coupling into account [22, 23]. All other computational parameters are unchanged compared to the study in the main text. In detail, we use the PBE functional [4] combined with the dhf-TZVP-2c basis sets [16]. A $k$ mesh of $32 \times 32$ is employed. A Gaussian smearing of 0.001 Hartree [24] and an SCF threshold of $10^{-8}$ Hartree are chosen. The electronic band structure is displayed in Figure 1.

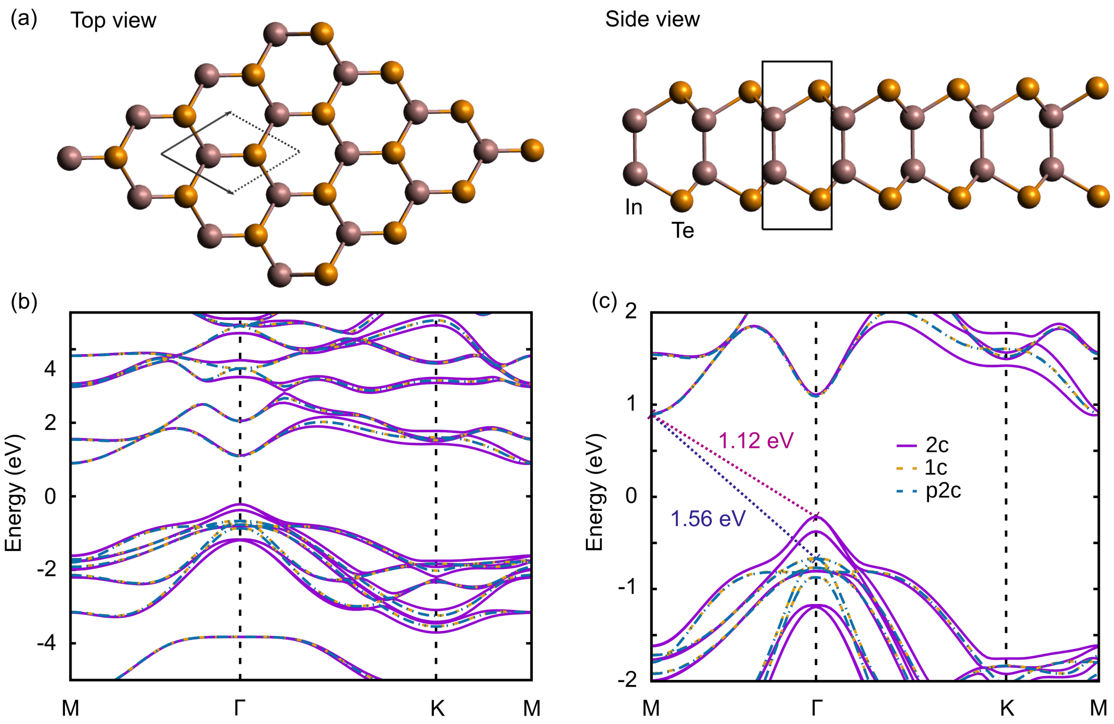


FIG. 1. (a) Top and side views of the two-dimensional InTe honeycomb system, with indicated unit cell. The unit cell consists of two In and two Te atoms. (b,c) Electronic band structure of the FBZ. The orange dashed lines are calculated without spin–orbit coupling in a one-component (1c) formalism, while the solid purple lines include spin–orbit interaction in the two-component (2c) methodology. The powder blue lines mark the two-component calculations with spin–orbit ECPs scaled to zero, i.e. the pseudo two-component (p2c) version. The black vertical dashed lines mark the Γ and K points of the Brillouin zone. Band gaps are indicated in blue (1c) and purple (2c) in panel (c).

Results with the HSE06 range-separated hybrid functional are shown in Figure 2. Here, unit cell parameters are optimized at the 2c PBE-D3-BJ level so that the structure is the same as that employed in the main text. The threshold of $5 \cdot 10^{-5}$ for the eigenvalues of the overlap matrix in the orthogonal basis transformation removes at most 4 linear combinations of basis functions (vectors). The total number of vectors is 232.

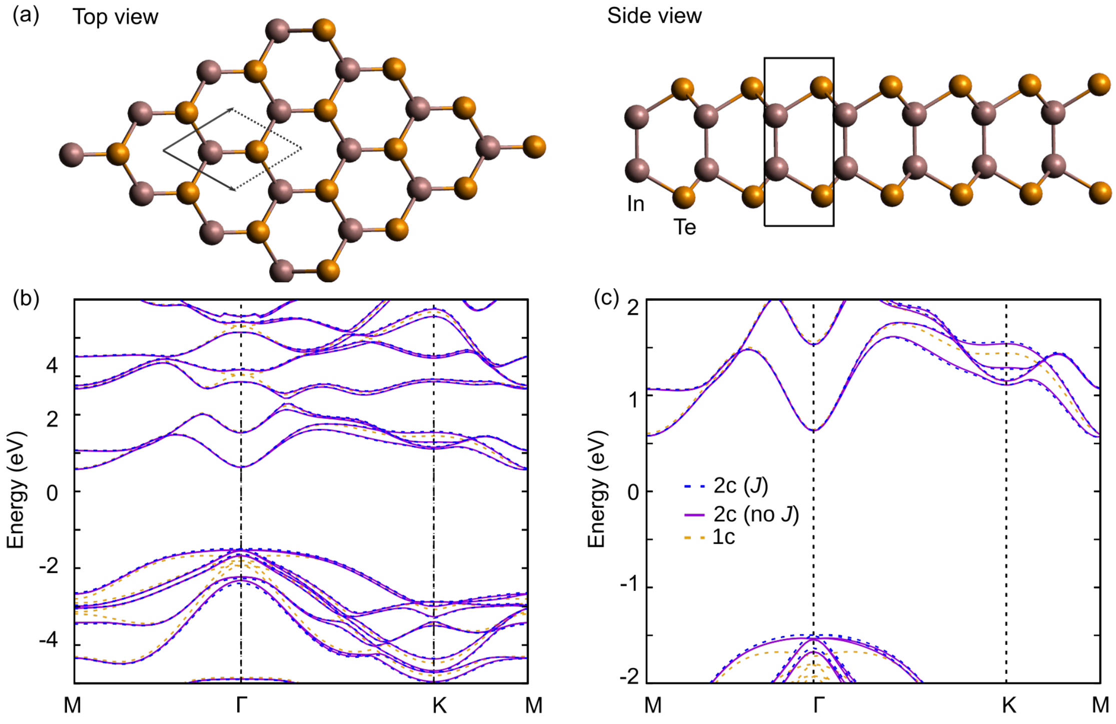


FIG. 2. (a) Top and side views of the two-dimensional InTe honeycomb system, with indicated unit cell. The unit cell consists of two In and two Te atoms. (b,c) Electronic band structure of the FBZ. The orange dashed lines are calculated without spin–orbit coupling in a one-component (1c) formalism, while the solid purple lines include spin–orbit interaction in the two-component (2c) methodology without the spin-current density contribution to the Fock exchange (2c no $J$). Dashed blue lines mark the two-component calculations with the complete 2c Fock exchange (2c $J$). The black vertical dashed lines mark the Γ and K points of the Brillouin zone.

## IV. ONE-DIMENSIONAL PLATINUM CHAINS

TABLE VII. Total SCF energies in Hartree obtained with the 1c RKS and 1c UKS formalisms and energies for the limit of a vanishing Gaussian smearing (limit). For the UKS calculations, the numbers of $\alpha$ and $\beta$ electrons are denoted by $n_\alpha$ and $n_\beta$. The $S_z$ expectation value is calculated as $\langle S_z \rangle = (n_\alpha - n_\beta)/2$. The PBE functional [4] is employed.

| $d$ | RKS limit | RKS | UKS limit | UKS | $n_\alpha$ | $n_\beta$ | $\langle S_z \rangle$ |
|---|---|---|---|---|---|---|---|
| 4.000 | −238.8565 | −238.8556 | −238.8565 | −238.8556 | 18.0000 | 18.0000 | $1.03 \times 10^{-5}$ |
| 4.100 | −238.9083 | −238.9074 | −238.9083 | −238.9074 | 18.0000 | 18.0000 | $1.86 \times 10^{-5}$ |
| 4.200 | −238.9467 | −238.9457 | −238.9467 | −238.9457 | 18.0000 | 18.0000 | $2.56 \times 10^{-5}$ |
| 4.300 | −238.9745 | −238.9733 | −238.9745 | −238.9733 | 18.0000 | 18.0000 | $3.89 \times 10^{-5}$ |
| 4.400 | −238.9936 | −238.9923 | −238.9936 | −238.9923 | 18.0001 | 17.9999 | $8.50 \times 10^{-5}$ |
| 4.500 | −239.0060 | −239.0045 | −239.0060 | −239.0045 | 18.0001 | 17.9999 | $1.10 \times 10^{-4}$ |
| 4.600 | −239.0131 | −239.0112 | −239.0131 | −239.0112 | 18.0003 | 17.9998 | $2.50 \times 10^{-4}$ |
| 4.700 | −239.0158 | −239.0137 | −239.0158 | −239.0137 | 18.0007 | 17.9993 | $7.02 \times 10^{-4}$ |
| 4.800 | −239.0153 | −239.0128 | −239.0153 | −239.0128 | 18.0007 | 17.9993 | $7.42 \times 10^{-4}$ |
| 4.900 | −239.0123 | −239.0093 | −239.0123 | −239.0093 | 18.0007 | 17.9994 | $6.48 \times 10^{-4}$ |
| 5.000 | −239.0073 | −239.0039 | −239.0073 | −239.0039 | 18.0008 | 17.9992 | $7.65 \times 10^{-4}$ |
| 5.020 | −239.0062 | −239.0026 | −239.0062 | −239.0026 | 18.0003 | 17.9997 | $2.59 \times 10^{-4}$ |
| 5.040 | −239.0049 | −239.0013 | −239.0049 | −239.0013 | 18.0004 | 17.9996 | $3.65 \times 10^{-4}$ |
| 5.060 | −239.0037 | −238.9999 | −239.0037 | −238.9999 | 18.0005 | 17.9995 | $5.38 \times 10^{-4}$ |
| 5.080 | −239.0023 | −238.9985 | −239.0023 | −238.9985 | 18.0008 | 17.9992 | $8.32 \times 10^{-4}$ |
| 5.100 | −239.0010 | −238.9970 | −239.0010 | −238.9970 | 18.0029 | 17.9971 | $2.93 \times 10^{-3}$ |
| 5.150 | −238.9974 | −238.9932 | −238.9974 | −238.9932 | 18.0158 | 17.9842 | $1.58 \times 10^{-2}$ |
| 5.200 | −238.9937 | −238.9892 | −238.9937 | −238.9892 | 18.2246 | 17.7754 | $2.25 \times 10^{-1}$ |
| 5.250 | −238.9897 | −238.9850 | −238.9899 | −238.9851 | 18.5527 | 17.4473 | $5.53 \times 10^{-1}$ |
| 5.300 | −238.9856 | −238.9806 | −238.9862 | −238.9814 | 18.7969 | 17.2031 | $7.97 \times 10^{-1}$ |
| 5.350 | −238.9815 | −238.9761 | −238.9828 | −238.9780 | 18.9539 | 17.0461 | $9.54 \times 10^{-1}$ |
| 5.400 | −238.9772 | −238.9716 | −238.9794 | −238.9747 | 19.0855 | 16.9145 | 1.09 |
| 5.500 | −238.9686 | −238.9625 | −238.9723 | −238.9674 | 19.1328 | 16.8672 | 1.13 |
| 5.600 | −238.9600 | −238.9533 | −238.9649 | −238.9598 | 19.1699 | 16.8302 | 1.17 |
| 5.700 | −238.9514 | −238.9442 | −238.9573 | −238.9519 | 19.1857 | 16.8143 | 1.19 |
| 5.800 | −238.9431 | −238.9353 | −238.9496 | −238.9439 | 19.1936 | 16.8064 | 1.19 |
| 5.900 | −238.9349 | −238.9267 | −238.9420 | −238.9359 | 19.1976 | 16.8024 | 1.20 |
| 6.000 | −238.9270 | −238.9184 | −238.9345 | −238.9281 | 19.1997 | 16.8003 | 1.20 |

TABLE VIII. Total SCF energies in Hartree obtained with the 2c KR, 2c canonical KU $S_z$, and 2c canonical KU $S_x$ approaches and energies for the limit of a vanishing Gaussian smearing (limit). Expectation values of the spin $S_{z,x}$ are listed for the open-shell calculations. The PBE functional [4] is employed.

| $d$ | KR limit | KR | KU $S_z$ limit | KU $S_z$ | $\langle S_z \rangle$ | KU $S_x$ limit | KU $S_x$ | $\langle S_x \rangle$ |
|---|---|---|---|---|---|---|---|---|
| 4.000 | −239.1439 | −239.1430 | −239.1439 | −239.1430 | $-2.86 \times 10^{-6}$ | −239.1439 | −239.1430 | $-1.12 \times 10^{-5}$ |
| 4.100 | −239.1956 | −239.1945 | −239.1956 | −239.1945 | $1.43 \times 10^{-6}$ | −239.1956 | −239.1945 | $-1.41 \times 10^{-5}$ |
| 4.200 | −239.2340 | −239.2325 | −239.2340 | −239.2325 | $1.69 \times 10^{-6}$ | −239.2340 | −239.2325 | $3.33 \times 10^{-5}$ |
| 4.300 | −239.2618 | −239.2601 | −239.2618 | −239.2601 | $1.10 \times 10^{-5}$ | −239.2618 | −239.2601 | $2.89 \times 10^{-5}$ |
| 4.400 | −239.2812 | −239.2792 | −239.2812 | −239.2792 | $2.23 \times 10^{-5}$ | −239.2812 | −239.2792 | $1.05 \times 10^{-4}$ |
| 4.500 | −239.2940 | −239.2916 | −239.2940 | −239.2916 | $7.31 \times 10^{-5}$ | −239.2940 | −239.2916 | $9.33 \times 10^{-5}$ |
| 4.600 | −239.3017 | −239.2988 | −239.3017 | −239.2988 | $9.94 \times 10^{-5}$ | −239.3017 | −239.2988 | $5.48 \times 10^{-4}$ |
| 4.700 | −239.3052 | −239.3019 | −239.3052 | −239.3019 | $1.23 \times 10^{-4}$ | −239.3052 | −239.3019 | $1.31 \times 10^{-3}$ |
| 4.800 | −239.3056 | −239.3019 | −239.3056 | −239.3019 | $5.67 \times 10^{-4}$ | −239.3056 | −239.3019 | $5.43 \times 10^{-3}$ |
| 4.900 | −239.3036 | −239.2994 | −239.3036 | −239.2994 | $-9.93 \times 10^{-4}$ | −239.3036 | −239.2994 | $6.00 \times 10^{-3}$ |
| 5.000 | −239.2998 | −239.2952 | −239.2998 | −239.2952 | $6.06 \times 10^{-5}$ | −239.2998 | −239.2952 | $2.23 \times 10^{-3}$ |
| 5.020 | −239.2989 | −239.2942 | −239.2989 | −239.2942 | $2.88 \times 10^{-5}$ | −239.2989 | −239.2942 | $8.09 \times 10^{-3}$ |
| 5.040 | −239.2979 | −239.2931 | −239.2979 | −239.2931 | $5.00 \times 10^{-5}$ | −239.2984 | −239.2939 | $3.91 \times 10^{-1}$ |
| 5.060 | −239.2969 | −239.2920 | −239.2969 | −239.2920 | $7.79 \times 10^{-5}$ | −239.2975 | −239.2930 | $4.33 \times 10^{-1}$ |
| 5.080 | −239.2958 | −239.2909 | −239.2958 | −239.2909 | $1.30 \times 10^{-4}$ | −239.2965 | −239.2921 | $4.69 \times 10^{-1}$ |
| 5.100 | −239.2947 | −239.2897 | −239.2947 | −239.2897 | $5.17 \times 10^{-4}$ | −239.2947 | −239.2911 | $4.96 \times 10^{-1}$ |
| 5.150 | −239.2918 | −239.2866 | −239.2918 | −239.2866 | $4.19 \times 10^{-3}$ | −239.2929 | −239.2884 | $5.63 \times 10^{-1}$ |
| 5.200 | −239.2887 | −239.2833 | −239.2887 | −239.2833 | $6.97 \times 10^{-3}$ | −239.2900 | −239.2855 | $6.14 \times 10^{-1}$ |
| 5.250 | −239.2855 | −239.2798 | −239.2855 | −239.2798 | $1.42 \times 10^{-2}$ | −239.2870 | −239.2824 | $6.56 \times 10^{-1}$ |
| 5.300 | −239.2821 | −239.2762 | −239.2821 | −239.2762 | $7.18 \times 10^{-2}$ | −239.2838 | −239.2790 | $6.92 \times 10^{-1}$ |
| 5.350 | −239.2785 | −239.2725 | −239.2786 | −239.2727 | $2.52 \times 10^{-1}$ | −239.2804 | −239.2755 | $7.22 \times 10^{-1}$ |
| 5.400 | −239.2749 | −239.2687 | −239.2753 | −239.2693 | $4.43 \times 10^{-1}$ | −239.2770 | −239.2719 | $7.48 \times 10^{-1}$ |
| 5.500 | −239.2676 | −239.2610 | −239.2684 | −239.2624 | $6.48 \times 10^{-1}$ | −239.2698 | −239.2645 | $7.95 \times 10^{-1}$ |
| 5.600 | −239.2600 | −239.2531 | −239.2613 | −239.2552 | $7.48 \times 10^{-1}$ | −239.2626 | −239.2569 | $8.41 \times 10^{-1}$ |
| 5.700 | −239.2525 | −239.2452 | −239.2541 | −239.2478 | $8.03 \times 10^{-1}$ | −239.2553 | −239.2493 | $8.83 \times 10^{-1}$ |
| 5.800 | −239.2450 | −239.2373 | −239.2469 | −239.2403 | $8.35 \times 10^{-1}$ | −239.2481 | −239.2418 | $9.23 \times 10^{-1}$ |
| 5.900 | −239.2376 | −239.2296 | −239.2398 | −239.2331 | $8.48 \times 10^{-1}$ | −239.2410 | −239.2345 | $9.55 \times 10^{-1}$ |
| 6.000 | −239.2303 | −239.2220 | −239.2329 | −239.2259 | $8.57 \times 10^{-1}$ | −239.2342 | −239.2274 | $9.80 \times 10^{-1}$ |

TABLE IX. Total SCF energies in Hartree obtained with the 2c KR and the 2c Scalmani–Frisch KU $S_x$ approaches and energies for the limit of a vanishing Gaussian smearing (limit). Expectation values of the spin $S_x$ are listed for the open-shell calculations. The PBE functional [4] is employed.

| $d$ | KR limit | KR | KU $S_x$ limit | KU $S_x$ | $\langle S_x \rangle$ |
|---|---|---|---|---|---|
| 4.000 | −239.1439 | −239.1430 | −239.1439 | −239.1430 | $4.48 \times 10^{-6}$ |
| 4.100 | −239.1956 | −239.1945 | −239.1956 | −239.1945 | $5.69 \times 10^{-6}$ |
| 4.200 | −239.2340 | −239.2325 | −239.2340 | −239.2325 | $9.80 \times 10^{-6}$ |
| 4.300 | −239.2618 | −239.2601 | −239.2618 | −239.2601 | $-7.77 \times 10^{-5}$ |
| 4.400 | −239.2812 | −239.2792 | −239.2812 | −239.2792 | $-3.60 \times 10^{-5}$ |
| 4.500 | −239.2940 | −239.2916 | −239.2940 | −239.2916 | $-3.62 \times 10^{-4}$ |
| 4.600 | −239.3017 | −239.2988 | −239.3017 | −239.2988 | $-3.39 \times 10^{-5}$ |
| 4.700 | −239.3052 | −239.3019 | −239.3052 | −239.3019 | $-1.41 \times 10^{-3}$ |
| 4.800 | −239.3056 | −239.3019 | −239.3056 | −239.3019 | $-4.09 \times 10^{-3}$ |
| 4.900 | −239.3036 | −239.2994 | −239.3036 | −239.2994 | $1.22 \times 10^{-2}$ |
| 5.000 | −239.2998 | −239.2952 | −239.3000 | −239.2956 | $2.89 \times 10^{-1}$ |
| 5.020 | −239.2989 | −239.2942 | −239.2992 | −239.2948 | $3.46 \times 10^{-1}$ |
| 5.040 | −239.2979 | −239.2931 | −239.2984 | −239.2940 | $3.93 \times 10^{-1}$ |
| 5.060 | −239.2969 | −239.2920 | −239.2975 | −239.2931 | $4.34 \times 10^{-1}$ |
| 5.080 | −239.2958 | −239.2909 | −239.2965 | −239.2921 | $4.70 \times 10^{-1}$ |
| 5.100 | −239.2947 | −239.2897 | −239.2955 | −239.2911 | $5.01 \times 10^{-1}$ |
| 5.150 | −239.2918 | −239.2866 | −239.2929 | −239.2884 | $5.66 \times 10^{-1}$ |
| 5.200 | −239.2887 | −239.2833 | −239.2900 | −239.2855 | $6.13 \times 10^{-1}$ |
| 5.250 | −239.2855 | −239.2798 | −239.2870 | −239.2824 | $6.57 \times 10^{-1}$ |
| 5.300 | −239.2821 | −239.2762 | −239.2838 | −239.2790 | $6.91 \times 10^{-1}$ |
| 5.350 | −239.2785 | −239.2725 | −239.2804 | −239.2755 | $7.19 \times 10^{-1}$ |
| 5.400 | −239.2749 | −239.2687 | −239.2770 | −239.2719 | $7.46 \times 10^{-1}$ |
| 5.500 | −239.2676 | −239.2610 | −239.2698 | −239.2645 | $7.92 \times 10^{-1}$ |
| 5.600 | −239.2600 | −239.2531 | −239.2626 | −239.2569 | $8.36 \times 10^{-1}$ |
| 5.700 | −239.2525 | −239.2452 | −239.2553 | −239.2493 | $8.77 \times 10^{-1}$ |
| 5.800 | −239.2450 | −239.2373 | −239.2481 | −239.2418 | $9.15 \times 10^{-1}$ |
| 5.900 | −239.2376 | −239.2296 | −239.2410 | −239.2345 | $9.47 \times 10^{-1}$ |
| 6.000 | −239.2303 | −239.2220 | −239.2342 | −239.2274 | $9.72 \times 10^{-1}$ |

TABLE X. Total SCF energies in Hartree obtained with the 1c RKS and 1c UKS formalisms and energies for the limit of a vanishing Gaussian smearing (limit). For the UKS calculations, the numbers of $\alpha$ and $\beta$ electrons are denoted by $n_\alpha$ and $n_\beta$. The $S_z$ expectation value is calculated as $\langle S_z \rangle = (n_\alpha - n_\beta)/2$. The S-VWN (V) functional [2, 3] is employed.

| $d$ | RKS limit | RKS | UKS limit | UKS | $n_\alpha$ | $n_\beta$ | $\langle S_z \rangle$ |
|---|---|---|---|---|---|---|---|
| 4.000 | −238.4885 | −238.4876 | −238.4885 | −238.4876 | 18.0000 | 18.0000 | 0.00 |
| 4.100 | −238.5363 | −238.5354 | −238.5363 | −238.5354 | 18.0000 | 18.0000 | $6.04 \times 10^{-14}$ |
| 4.200 | −238.5708 | −238.5698 | −238.5708 | −238.5698 | 18.0000 | 18.0000 | $1.86 \times 10^{-5}$ |
| 4.300 | −238.5949 | −238.5937 | −238.5949 | −238.5937 | 18.0000 | 18.0000 | $2.72 \times 10^{-5}$ |
| 4.400 | −238.6105 | −238.6091 | −238.6105 | −238.6091 | 18.0000 | 18.0000 | $4.46 \times 10^{-5}$ |
| 4.500 | −238.6195 | −238.6179 | −238.6195 | −238.6179 | 18.0001 | 17.9999 | $8.67 \times 10^{-5}$ |
| 4.600 | −238.6233 | −238.6214 | −238.6233 | −238.6214 | 18.0002 | 17.9998 | $2.02 \times 10^{-4}$ |
| 4.700 | −238.6230 | −238.6207 | −238.6230 | −238.6207 | 18.0006 | 17.9994 | $5.97 \times 10^{-4}$ |
| 4.800 | −238.6196 | −238.6169 | −238.6196 | −238.6169 | 18.0009 | 17.9991 | $9.02 \times 10^{-4}$ |
| 4.900 | −238.6138 | −238.6106 | −238.6138 | −238.6106 | 18.0011 | 17.9989 | $1.14 \times 10^{-3}$ |
| 5.000 | −238.6062 | −238.6026 | −238.6062 | −238.6026 | 18.0010 | 17.9990 | $1.03 \times 10^{-3}$ |
| 5.100 | −238.5973 | −238.5932 | −238.5973 | −238.5932 | 18.0006 | 17.9994 | $5.63 \times 10^{-4}$ |
| 5.200 | −238.5876 | −238.5829 | −238.5876 | −238.5829 | 18.0674 | 17.9326 | $6.74 \times 10^{-2}$ |
| 5.300 | −238.5773 | −238.5721 | −238.5775 | −238.5724 | 18.5460 | 17.4540 | $5.46 \times 10^{-1}$ |
| 5.400 | −238.5667 | −238.5609 | −238.5679 | −238.5627 | 18.9002 | 17.0998 | $9.00 \times 10^{-1}$ |
| 5.500 | −238.5561 | −238.5497 | −238.5587 | −238.5534 | 19.0715 | 16.9285 | 1.07 |
| 5.600 | −238.5455 | −238.5386 | −238.5494 | −238.5440 | 19.1478 | 16.8522 | 1.15 |
| 5.700 | −238.5351 | −238.5276 | −238.5400 | −238.5344 | 19.1842 | 16.8158 | 1.18 |
| 5.800 | −238.5249 | −238.5170 | −238.5307 | −238.5248 | 19.2022 | 16.7978 | 1.20 |
| 5.900 | −238.5151 | −238.5067 | −238.5215 | −238.5153 | 19.2111 | 16.7889 | 1.21 |
| 6.000 | −238.5056 | −238.4967 | −238.5125 | −238.5059 | 19.2159 | 16.7841 | 1.22 |

TABLE XI. Total SCF energies in Hartree obtained with the 2c KR, 2c canonical KU $S_z$, and 2c canonical KU $S_x$ approaches and energies for the limit of a vanishing Gaussian smearing (limit). Expectation values of the spin $S_{z,x}$ are listed for the open-shell calculations. The S-VWN (V) functional [2, 3] is employed.

| $d$ | KR limit | KR | KU $S_z$ limit | KU $S_z$ | $\langle S_z \rangle$ | KU $S_x$ limit | KU $S_x$ | $\langle S_x \rangle$ |
|---|---|---|---|---|---|---|---|---|
| 4.000 | −238.7779 | −238.7769 | −238.7779 | −238.7769 | $-1.60 \times 10^{-6}$ | −238.7779 | −238.7769 | $4.58 \times 10^{-5}$ |
| 4.100 | −238.8256 | −238.8243 | −238.8256 | −238.8243 | $1.82 \times 10^{-5}$ | −238.8256 | −238.8243 | $2.79 \times 10^{-5}$ |
| 4.200 | −238.8601 | −238.8586 | −238.8601 | −238.8586 | $-3.67 \times 10^{-9}$ | −238.8601 | −238.8586 | $2.74 \times 10^{-5}$ |
| 4.300 | −238.8844 | −238.8825 | −238.8844 | −238.8825 | $6.47 \times 10^{-8}$ | −238.8844 | −238.8825 | $2.01 \times 10^{-4}$ |
| 4.400 | −238.9004 | −238.8982 | −238.9004 | −238.8982 | $1.80 \times 10^{-7}$ | −238.9004 | −238.8982 | $-4.26 \times 10^{-4}$ |
| 4.500 | −238.9099 | −238.9074 | −238.9099 | −238.9074 | $-2.01 \times 10^{-6}$ | −238.9099 | −238.9074 | $6.26 \times 10^{-4}$ |
| 4.600 | −238.9144 | −238.9115 | −238.9144 | −238.9115 | $-1.79 \times 10^{-6}$ | −238.9144 | −238.9115 | $1.23 \times 10^{-3}$ |
| 4.700 | −238.9149 | −238.9116 | −238.9149 | −238.9116 | $1.38 \times 10^{-8}$ | −238.9149 | −238.9116 | $1.71 \times 10^{-3}$ |
| 4.800 | −238.9125 | −238.9087 | −238.9125 | −238.9087 | $2.03 \times 10^{-3}$ | −238.9125 | −238.9087 | $8.34 \times 10^{-4}$ |
| 4.900 | −238.9077 | −238.9035 | −238.9077 | −238.9035 | $1.12 \times 10^{-3}$ | −238.9077 | −238.9035 | $3.68 \times 10^{-3}$ |
| 5.000 | −238.9013 | −238.8967 | −238.9013 | −238.8967 | $1.09 \times 10^{-3}$ | −238.9014 | −238.8967 | $1.71 \times 10^{-2}$ |
| 5.100 | −238.8938 | −238.8887 | −238.8938 | −238.8887 | $1.01 \times 10^{-3}$ | −238.8939 | −238.8890 | $2.60 \times 10^{-1}$ |
| 5.200 | −238.8854 | −238.8799 | −238.8854 | −238.8799 | $2.94 \times 10^{-3}$ | −238.8861 | −238.8811 | $4.83 \times 10^{-1}$ |
| 5.300 | −238.8765 | −238.8706 | −238.8765 | −238.8706 | $5.99 \times 10^{-3}$ | −238.8776 | −238.8725 | $6.02 \times 10^{-1}$ |
| 5.400 | −238.8672 | −238.8609 | −238.8672 | −238.8609 | $3.43 \times 10^{-2}$ | −238.8686 | −238.8634 | $6.82 \times 10^{-1}$ |
| 5.500 | −238.8578 | −238.8511 | −238.8579 | −238.8513 | $2.58 \times 10^{-1}$ | −238.8595 | −238.8540 | $7.42 \times 10^{-1}$ |
| 5.600 | −238.8483 | −238.8413 | −238.8488 | −238.8422 | $5.32 \times 10^{-1}$ | −238.8503 | −238.8445 | $7.96 \times 10^{-1}$ |
| 5.700 | −238.8390 | −238.8316 | −238.8398 | −238.8330 | $6.56 \times 10^{-1}$ | −238.8412 | −238.8351 | $8.41 \times 10^{-1}$ |
| 5.800 | −238.8297 | −238.8220 | −238.8309 | −238.8239 | $7.27 \times 10^{-1}$ | −238.8322 | −238.8258 | $8.83 \times 10^{-1}$ |
| 5.900 | −238.8207 | −238.8126 | −238.8221 | −238.8150 | $7.72 \times 10^{-1}$ | −238.8235 | −238.8169 | $9.19 \times 10^{-1}$ |
| 6.000 | −238.8119 | −238.8035 | −238.8136 | −238.8062 | $8.03 \times 10^{-1}$ | −238.8151 | −238.8082 | $9.50 \times 10^{-1}$ |

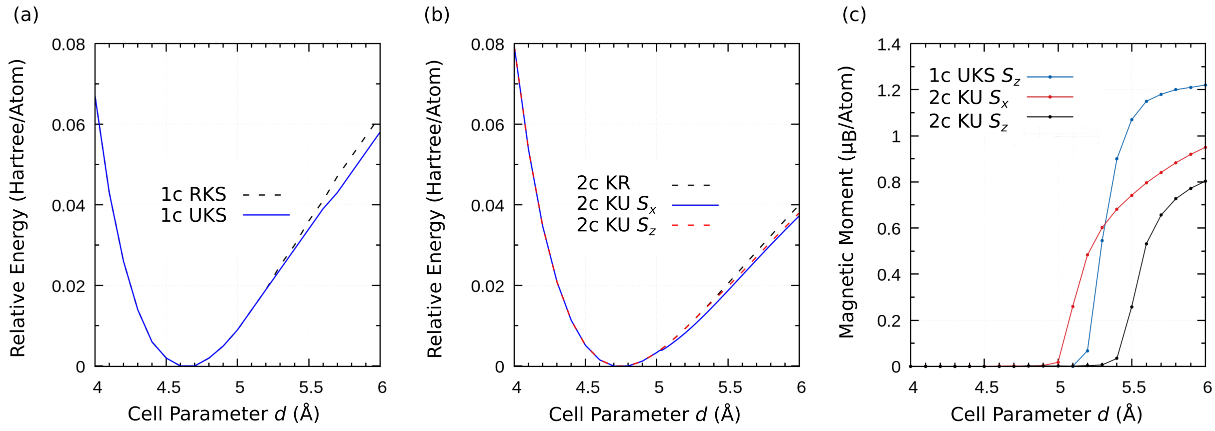


FIG. 3. (a) Dependence of the energy on the cell parameter in units of Hartree per atom for the 1c RKS and 1c UKS calculations with the S-VWN (V) functional [2, 3] and the dhf-SVP-2c basis set [16] combined with small-core Dirac–Fock ECPs [25]. (b) Dependence of the energy on the cell parameter in units of Hartree per atom for the 2c KR, 2c KU $S_x$, and 2c KU $S_z$ calculations. (c) Magnetic moment in units of Bohr's magneton $\mu_\mathrm{B}$ per atom for the spin contribution of the 1c UKS, 2c KU $S_x$, and 2c KU $S_z$ calculations.

TABLE XII. Total SCF energies in Hartree obtained with the 1c RKS and 1c UKS formalisms and energies for the limit of a vanishing Gaussian smearing (limit). For the UKS calculations, the numbers of $\alpha$ and $\beta$ electrons are denoted by $n_\alpha$ and $n_\beta$. The $S_z$ expectation value is calculated as $\langle S_z \rangle = (n_\alpha - n_\beta)/2$. The TPSS functional [6] is employed.

| $d$ | RKS limit | RKS | UKS limit | UKS | $n_\alpha$ | $n_\beta$ | $\langle S_z \rangle$ |
|---|---|---|---|---|---|---|---|
| 4.000 | −238.7223 | −238.7214 | −238.7223 | −238.7214 | 18.0000 | 18.0000 | $1.30 \times 10^{-5}$ |
| 4.100 | −238.7742 | −238.7732 | −238.7742 | −238.7732 | 18.0000 | 18.0000 | $2.46 \times 10^{-5}$ |
| 4.200 | −238.8125 | −238.8115 | −238.8125 | −238.8115 | 18.0000 | 18.0000 | $3.56 \times 10^{-5}$ |
| 4.300 | −238.8401 | −238.8389 | −238.8401 | −238.8389 | 18.0001 | 17.9999 | $7.48 \times 10^{-5}$ |
| 4.400 | −238.8590 | −238.8577 | −238.8590 | −238.8577 | 18.0001 | 17.9999 | $1.27 \times 10^{-4}$ |
| 4.500 | −238.8711 | −238.8696 | −238.8711 | −238.8696 | 18.0002 | 17.9997 | $2.48 \times 10^{-4}$ |
| 4.600 | −238.8778 | −238.8760 | −238.8778 | −238.8760 | 18.0005 | 17.9995 | $5.20 \times 10^{-4}$ |
| 4.700 | −238.8803 | −238.8782 | −238.8803 | −238.8782 | 18.0014 | 17.9986 | $1.41 \times 10^{-3}$ |
| 4.800 | −238.8794 | −238.8769 | −238.8794 | −238.8769 | 18.0009 | 17.9991 | $9.09 \times 10^{-4}$ |
| 4.900 | −238.8760 | −238.8731 | −238.8760 | −238.8731 | 18.0006 | 17.9995 | $5.48 \times 10^{-4}$ |
| 5.000 | −238.8706 | −238.8673 | −238.8706 | −238.8673 | 18.0004 | 17.9996 | $3.93 \times 10^{-4}$ |
| 5.100 | −238.8638 | −238.8600 | −238.8638 | −238.8600 | 18.0209 | 17.9791 | $2.09 \times 10^{-2}$ |
| 5.200 | −238.8561 | −238.8518 | −238.8562 | −238.8519 | 18.5396 | 17.4604 | $5.40 \times 10^{-1}$ |
| 5.300 | −238.8477 | −238.8428 | −238.8491 | −238.8446 | 19.0238 | 16.9762 | 1.02 |
| 5.400 | −238.8388 | −238.8334 | −238.8421 | −238.8377 | 19.1479 | 16.8521 | 1.15 |
| 5.500 | −238.8298 | −238.8239 | −238.8347 | −238.8302 | 19.1888 | 16.8112 | 1.19 |
| 5.600 | −238.8208 | −238.8143 | −238.8270 | −238.8222 | 19.2055 | 16.7945 | 1.21 |
| 5.700 | −238.8119 | −238.8048 | −238.8190 | −238.8139 | 19.2133 | 16.7867 | 1.21 |
| 5.800 | −238.8031 | −238.7955 | −238.8111 | −238.8057 | 19.2192 | 16.7808 | 1.22 |
| 5.900 | −238.7946 | −238.7866 | −238.8033 | −238.7976 | 19.2244 | 16.7756 | 1.22 |
| 6.000 | −238.7865 | −238.7780 | −238.7957 | −238.7896 | 19.2293 | 16.7707 | 1.23 |

TABLE XIII. Total SCF energies in Hartree obtained with the 2c KR, 2c canonical KU $S_z$, and 2c canonical KU $S_x$ approaches and energies for the limit of a vanishing Gaussian smearing (limit). Expectation values of the spin $S_{z,x}$ are listed for the open-shell calculations. The TPSS functional [6] is employed.

| $d$ | KR limit | KR | KU $S_z$ limit | KU $S_z$ | $\langle S_z \rangle$ | KU $S_x$ limit | KU $S_x$ | $\langle S_x \rangle$ |
|---|---|---|---|---|---|---|---|---|
| 4.000 | −239.0074 | −239.0065 | −239.0074 | −239.0065 | $1.83 \times 10^{-5}$ | −239.0074 | −239.0065 | $3.62 \times 10^{-5}$ |
| 4.100 | −239.0592 | −239.0580 | −239.0592 | −239.0580 | $2.64 \times 10^{-5}$ | −239.0592 | −239.0580 | $2.35 \times 10^{-5}$ |
| 4.200 | −239.0975 | −239.0961 | −239.0975 | −239.0961 | $1.67 \times 10^{-5}$ | −239.0975 | −239.0961 | $4.72 \times 10^{-5}$ |
| 4.300 | −239.1251 | −239.1234 | −239.1251 | −239.1234 | $4.79 \times 10^{-5}$ | −239.1251 | −239.1234 | $3.41 \times 10^{-4}$ |
| 4.400 | −239.1443 | −239.1423 | −239.1443 | −239.1423 | $1.92 \times 10^{-4}$ | −239.1443 | −239.1423 | $4.77 \times 10^{-4}$ |
| 4.500 | −239.1568 | −239.1544 | −239.1568 | −239.1544 | $1.57 \times 10^{-4}$ | −239.1568 | −239.1544 | $5.10 \times 10^{-4}$ |
| 4.600 | −239.1641 | −239.1613 | −239.1641 | −239.1613 | $2.10 \times 10^{-4}$ | −239.1641 | −239.1613 | $5.05 \times 10^{-4}$ |
| 4.700 | −239.1672 | −239.1640 | −239.1672 | −239.1640 | $1.81 \times 10^{-4}$ | −239.1672 | −239.1640 | $3.94 \times 10^{-4}$ |
| 4.800 | −239.1672 | −239.1636 | −239.1672 | −239.1636 | $1.93 \times 10^{-4}$ | −239.1672 | −239.1636 | $3.97 \times 10^{-3}$ |
| 4.900 | −239.1648 | −239.1607 | −239.1648 | −239.1607 | $1.10 \times 10^{-4}$ | −239.1650 | −239.1611 | $2.54 \times 10^{-1}$ |
| 5.000 | −239.1606 | −239.1560 | −239.1606 | −239.1560 | $1.31 \times 10^{-3}$ | −239.1614 | −239.1575 | $4.91 \times 10^{-1}$ |
| 5.100 | −239.1550 | −239.1501 | −239.1550 | −239.1501 | $6.56 \times 10^{-3}$ | −239.1565 | −239.1525 | $6.27 \times 10^{-1}$ |
| 5.200 | −239.1486 | −239.1432 | −239.1487 | −239.1434 | $1.21 \times 10^{-1}$ | −239.1506 | −239.1464 | $7.13 \times 10^{-1}$ |
| 5.300 | −239.1415 | −239.1357 | −239.1419 | −239.1365 | $5.13 \times 10^{-1}$ | −239.1439 | −239.1395 | $7.76 \times 10^{-1}$ |
| 5.400 | −239.1340 | −239.1278 | −239.1352 | −239.1299 | $7.27 \times 10^{-1}$ | −239.1367 | −239.1320 | $8.30 \times 10^{-1}$ |
| 5.500 | −239.1262 | −239.1197 | −239.1283 | −239.1231 | $8.06 \times 10^{-1}$ | −239.1293 | −239.1241 | $8.84 \times 10^{-1}$ |
| 5.600 | −239.1183 | −239.1115 | −239.1210 | −239.1157 | $8.55 \times 10^{-1}$ | −239.1217 | −239.1162 | $9.27 \times 10^{-1}$ |
| 5.700 | −239.1104 | −239.1032 | −239.1136 | −239.1081 | $8.78 \times 10^{-1}$ | −239.1141 | −239.1083 | $9.69 \times 10^{-1}$ |
| 5.800 | −239.1025 | −239.0950 | −239.1062 | −239.1005 | $8.91 \times 10^{-1}$ | −239.1067 | −239.1006 | 1.00 |
| 5.900 | −239.0948 | −239.0869 | −239.0989 | −239.0929 | $8.97 \times 10^{-1}$ | −239.0994 | −239.0931 | 1.03 |
| 6.000 | −239.0873 | −239.0791 | −239.0916 | −239.0853 | $8.89 \times 10^{-1}$ | −239.0924 | −239.0859 | 1.04 |

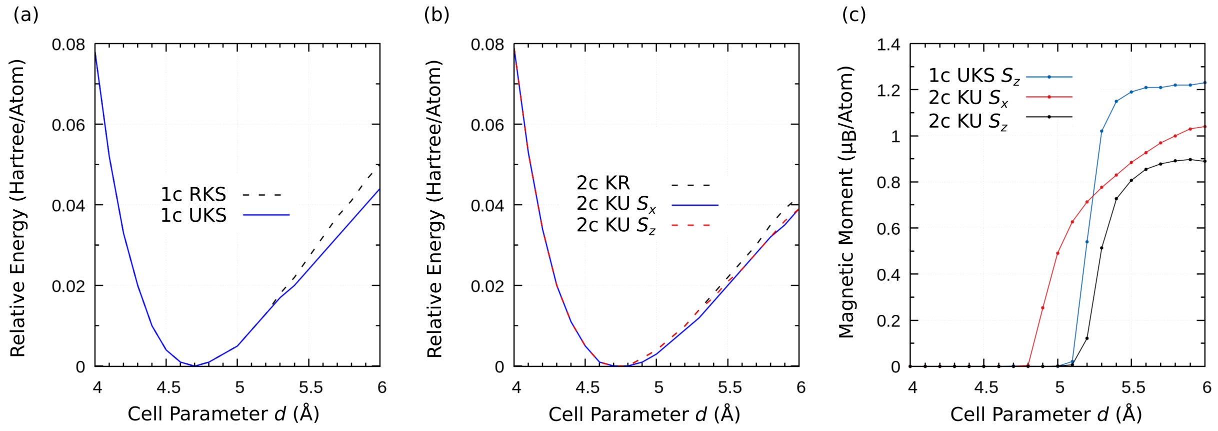


FIG. 4. (a) Dependence of the energy on the cell parameter in units of Hartree per atom for the 1c RKS and 1c UKS calculations with the TPSS functional [6] and the dhf-SVP-2c basis set [16] combined with small-core Dirac–Fock ECPs [25]. (b) Dependence of the energy on the cell parameter in units of Hartree per atom for the 2c KR, 2c KU $S_x$, and 2c KU $S_z$ calculations. (c) Magnetic moment in units of Bohr's magneton $\mu_{\mathrm{B}}$ per atom for the spin contribution of the 1c UKS, 2c KU $S_x$, and 2c KU $S_z$ calculations.

TABLE XIV. Total SCF energies in Hartree with the 1c RKS and 1c UKS formalisms and energies for the limit of a vanishing Gaussian smearing (limit). For the UKS calculations, the numbers of $\alpha$ and $\beta$ electrons are denoted by $n_\alpha$ and $n_\beta$. The $S_z$ expectation value is calculated as $\langle S_z \rangle = (n_\alpha - n_\beta)/2$. The HSE06 functional [26–28] is used with a threshold of $5 \cdot 10^{-5}$ for the eigenvalues of the overlap matrix in the orthogonal basis transformation for $d = 4.0$ to $d = 4.7$Å. This removes at most 2 linear combinations of basis functions (vectors), total number of vectors is 86. For the other structures, the default threshold of $10^{-6}$ is applied. 33 $k$ points are employed throughout.

| $d$ | RKS limit | RKS | UKS limit | UKS | $n_\alpha$ | $n_\beta$ | $\langle S_z \rangle$ |
|---|---|---|---|---|---|---|---|
| 4.000 | −238.7081 | −238.7073 | −238.7081 | −238.7073 | 18.0000 | 18.0000 | $5.18 \times 10^{-8}$ |
| 4.100 | −238.7576 | −238.7568 | −238.7576 | −238.7568 | 18.0000 | 18.0000 | $1.82 \times 10^{-7}$ |
| 4.200 | −238.7939 | −238.7930 | −238.7939 | −238.7930 | 18.0000 | 18.0000 | $5.88 \times 10^{-7}$ |
| 4.300 | −238.8197 | −238.8187 | −238.8197 | −238.8187 | 18.0000 | 18.0000 | $2.54 \times 10^{-6}$ |
| 4.400 | −238.8370 | −238.8358 | −238.8370 | −238.8358 | 18.0000 | 18.0000 | $2.26 \times 10^{-5}$ |
| 4.500 | −238.8476 | −238.8464 | −238.8476 | −238.8464 | 18.0002 | 17.9998 | $1.76 \times 10^{-4}$ |
| 4.600 | −238.8531 | −238.8517 | −238.8531 | −238.8517 | 18.0048 | 17.9952 | $4.82 \times 10^{-3}$ |
| 4.700 | −238.8545 | −238.8529 | −238.8566 | −238.8554 | 18.3843 | 17.6157 | $3.84 \times 10^{-1}$ |
| 4.800 | −238.8530 | −238.8512 | −238.8556 | −238.8543 | 18.4481 | 17.5518 | $4.48 \times 10^{-1}$ |
| 4.900 | −238.8488 | −238.8467 | −238.8550 | −238.8541 | 19.1415 | 16.8585 | 1.14 |
| 5.000 | −238.8430 | −238.8407 | −238.8532 | −238.8523 | 19.1571 | 16.8429 | 1.16 |
| 5.100 | −238.8361 | −238.8337 | −238.8494 | −238.8484 | 19.1669 | 16.8331 | 1.17 |
| 5.200 | −238.8286 | −238.8262 | −238.8470 | −238.8465 | 19.2274 | 16.7726 | 1.23 |
| 5.300 | −238.8205 | −238.8182 | −238.8422 | −238.8417 | 19.2330 | 16.7670 | 1.23 |
| 5.400 | −238.8120 | −238.8097 | −238.8331 | −238.8323 | 19.2724 | 16.7276 | 1.27 |
| 5.500 | −238.8033 | −238.8007 | −238.8311 | −238.8306 | 19.2418 | 16.7582 | 1.24 |
| 5.600 | −238.7944 | −238.7916 | −238.8253 | −238.8247 | 19.2461 | 16.7539 | 1.25 |
| 5.700 | −238.7856 | −238.7824 | −238.8195 | −238.8188 | 19.2510 | 16.7490 | 1.25 |
| 5.800 | −238.7851 | −238.7830 | −238.8137 | −238.8130 | 19.2564 | 16.7436 | 1.26 |
| 5.900 | −238.7788 | −238.7766 | −238.8080 | −238.8072 | 19.2417 | 16.7583 | 1.24 |
| 6.000 | −238.7724 | −238.7700 | −238.8060 | −238.8051 | 19.1536 | 16.8464 | 1.15 |

## V. STRUCTURES

Geometric structures are given in TURBOMOLE format [29–32]. Cell parameters ($cell) are specified in atomic units unless stated differently, i.e. angs for Ångström. Coordinates inside the cell are given in atomic units ($coord) or with fractional and dimensionless units ($coord frac). Structures are listed under the subsection headlines of the main text, where they are used.

### A. SCF Computation Times

```
$cell
 6.61460836 6.61460836 6.61460836 60.0 60.0 60.0
$coord
    0.00000000000000       0.00000000000000       0.00000000000000      pb
$end
```

## B. Ionization Energies of Zero-Dimensional Heavy $p$-Block Atoms

```
$coord
    0.00000000000000      0.00000000000000      0.00000000000000      in
$end

$coord
    0.00000000000000      0.00000000000000      0.00000000000000      sn
$end

$coord
    0.00000000000000      0.00000000000000      0.00000000000000      sb
$end

$coord
    0.00000000000000      0.00000000000000      0.00000000000000      te
$end

$coord
    0.00000000000000      0.00000000000000      0.00000000000000      i
$end

$coord
    0.00000000000000      0.00000000000000      0.00000000000000      tl
$end

$coord
    0.00000000000000      0.00000000000000      0.00000000000000      pb
$end

$coord
    0.00000000000000      0.00000000000000      0.00000000000000      bi
$end

$coord
    0.00000000000000      0.00000000000000      0.00000000000000      po
$end

$coord
    0.00000000000000      0.00000000000000      0.00000000000000      at
$end
```

## C. Band Structures of Three-Dimensional Gold and Lead Crystals

```
a) Three-dimensional gold fcc crystal
$cell
 5.45185 5.45185 5.45185 60.0 60.0 60.0
$coord
    0.00000000000000      0.00000000000000      0.00000000000000      au
$end
```

```
b) Three-dimensional lead fcc crystal
$cell
 6.57429 6.57429 6.57429 60.0 60.0 60.0
$coord
    0.00000000000000      0.00000000000000      0.00000000000000      pb
$end
```

## D. Band Gaps of Three-Dimensional Silver Halide Crystals

a) Non-relaxed structures

i) AgCl

```
$cell angs
   3.9683   3.9683   3.9683  60.0000   60.0000   60.0000
$coord frac
    0.00000000000000      0.00000000000000      0.00000000000000      ag
    0.50000000000000      0.50000000000000      0.50000000000000      cl
$end
```

ii) AgBr

```
$cell angs
   4.1316   4.1316   4.1316  60.0000   60.0000   60.0000
$coord frac
    0.00000000000000      0.00000000000000      0.00000000000000      ag
    0.50000000000000      0.50000000000000      0.50000000000000      br
$end
```

iii) AgI

```
$cell angs
   4.3621   4.3621   4.3621   60.0000   60.0000   60.0000
$coord frac
    0.00000000000000      0.00000000000000      0.00000000000000      ag
    0.50000000000000      0.50000000000000      0.50000000000000      i
$end
```

b) Relaxed structures without D3-BJ

i) AgCl

SVWN (V)

```
$cell  angs
  3.84825344503333333333   3.84825344503333333333   3.84825344503333333333   60.0  60.0  60.0
$coord frac
    0.00000000000000      0.00000000000000      0.00000000000000  ag
    0.50000000000000      0.50000000000000      0.50000000000000  cl
$end
```

PBE

```
$cell  angs
  3.97881790756666666666   3.97881790756666666666   3.97881790756666666666   60.0   60.0   60.0
$coord frac
    0.00000000000000      0.00000000000000      0.00000000000000  ag
    0.50000000000000      0.50000000000000      0.50000000000000  cl
$end
```

PBEsol

```
$cell  angs
   3.90080049883333333333   3.90080049883333333333   3.90080049883333333333   60.0   60.0   60.0
$coord frac
    0.00000000000000      0.00000000000000      0.00000000000000  ag
    0.50000000000000      0.50000000000000      0.50000000000000  cl
$end
```

TPSS

```
$cell  angs
   3.95192791410000000000   3.95192791410000000000   3.95192791410000000000   60.0   60.0   60.0
$coord frac
    0.00000000000000      0.00000000000000      0.00000000000000  ag
    0.50000000000000      0.50000000000000      0.50000000000000  cl
$end
```

revTPSS

```
$cell  angs
    3.93323644336667     3.93323644336667     3.93323644336667    60.0    60.0    60.0
$coord frac
    0.00000000000000      0.00000000000000      0.00000000000000  ag
    0.50000000000000      0.50000000000000      0.50000000000000  cl
$end
```

```
Tao-Mo
$cell  angs
   3.9184690781   3.9184690781   3.9184690781  60.0   60.0   60.0
$coord frac
    0.00000000000000      0.00000000000000      0.00000000000000  ag
    0.50000000000000      0.50000000000000      0.50000000000000  cl
$end

PKZB
$cell  angs
   3.9880650068   3.9880650068   3.9880650068   60.0   60.0   60.0
$coord frac
    0.00000000000000      0.00000000000000      0.00000000000000  ag
    0.50000000000000      0.50000000000000      0.50000000000000  cl
$end

r2SCAN
$cell  angs
   3.94398068143333333333   3.94398068143333333333   3.94398068143333333333   60.0    60.0   60.0
$coord frac
    0.00000000000000      0.00000000000000      0.00000000000000  ag
    0.50000000000000      0.50000000000000      0.50000000000000  cl
$end

2c-SVWN (V)
$cell  angs
    3.8017642716     3.8017642716     3.8017642716    60.0    60.0  60.0
$coord frac
    0.00000000000000      0.00000000000000      0.00000000000000  ag
    0.50000000000000      0.50000000000000      0.50000000000000  cl
$end

2c-PBE
$cell  angs
    3.97687054476666666666   3.97687054476666666666   3.97687054476666666666  60.0 60.0 60.0
$coord frac
    0.00000000000000      0.00000000000000      0.00000000000000  ag
    0.50000000000000      0.50000000000000      0.50000000000000  cl
$end

2c-PBEsol
$cell  angs
    3.89940465353333333333  3.89940465353333333333   3.89940465353333333333  60.0  60.0  60.0
$coord frac
    0.00000000000000      0.00000000000000      0.00000000000000  ag
    0.50000000000000      0.50000000000000      0.50000000000000  cl
$end
```

```
2c-TPSS
$cell  angs
   3.95007142833333333333  3.95007142833333333333  3.95007142833333333333  60.0   60.0  60.0
$coord frac
   0.00000000000000      0.00000000000000      0.00000000000000  ag
   0.50000000000000      0.50000000000000      0.50000000000000  cl
$end

2c-revTPSS
$cell  angs
   3.93227899606666666666  3.93227899606666666666   3.93227899606666666666  60.0  60.0  60.0
$coord frac
   0.00000000000000      0.00000000000000      0.00000000000000  ag
   0.50000000000000      0.50000000000000      0.50000000000000  cl
$end

2c-Tao-Mo
$cell  angs
  3.91842787876666666666  3.91842787876666666666  3.91842787876666666666 60.0  60.0  60.0
$coord frac
   0.00000000000000      0.00000000000000      0.00000000000000  ag
   0.50000000000000      0.50000000000000      0.50000000000000  cl
$end

2c-PKZB
$cell  angs
   3.9852599056     3.9852599056     3.9852599056    60.0   60.0   60.0
$coord frac
   0.00000000000000      0.00000000000000      0.00000000000000  ag
   0.50000000000000      0.50000000000000      0.50000000000000  cl
$end

2c-r2SCAN
$cell  angs
   3.9430444896     3.9430444896     3.9430444896    60.0    60.0    60.0
$coord frac
   0.00000000000000      0.00000000000000      0.00000000000000  ag
   0.50000000000000      0.50000000000000      0.50000000000000  cl
$end
```

ii) AgBr

```
SVWN (V)
$cell  angs
   3.9659229888   3.9659229888   3.9659229888  60.0   60.0  60.0
$coord frac
    0.00000000000000      0.00000000000000      0.00000000000000  ag
    0.50000000000000      0.50000000000000      0.50000000000000  br
$end

PBE
$cell  angs
   4.13768026056666666666  4.13768026056666666666  4.13768026056666666666  60.0  60.0  60.0
$coord frac
    0.00000000000000      0.00000000000000      0.00000000000000  ag
    0.50000000000000      0.50000000000000      0.50000000000000  br
$end

PBEsol
$cell  angs
  4.02721811653333333333  4.02721811653333333333  4.02721811653333333333  60.0  60.0  60.0
$coord frac
    0.00000000000000      0.00000000000000      0.00000000000000  ag
    0.50000000000000      0.50000000000000      0.50000000000000  br
$end

TPSS
$cell  angs
  4.11184283506666666666  4.11184283506666666666  4.11184283506666666666  60.0  60.0  60.0
$coord frac
    0.00000000000000      0.00000000000000      0.00000000000000  ag
    0.50000000000000      0.50000000000000      0.50000000000000  br
$end

revTPSS
$cell  angs
  4.09371116283333333333  4.09371116283333333333  4.09371116283333333333  60.0  60.0  60.0
$coord frac
    0.00000000000000      0.00000000000000      0.00000000000000  ag
    0.50000000000000      0.50000000000000      0.50000000000000  br
$end
```

```
Tao-Mo
$cell  angs
  4.08238349393333333333  4.08238349393333333333  4.08238349393333333333  60.0  60.0  60.0
$coord frac
    0.00000000000000      0.00000000000000      0.00000000000000  ag
    0.50000000000000      0.50000000000000      0.50000000000000  br
$end

PKZB
$cell  angs
  4.14890441196666666666  4.14890441196666666666  4.14890441196666666666  60.0 60.0 60.0
$coord frac
    0.00000000000000      0.00000000000000      0.00000000000000  ag
    0.50000000000000      0.50000000000000      0.50000000000000  br
$end

r2SCAN
$cell  angs
  4.11077895733333333333  4.11077895733333333333  4.11077895733333333333  60.0  60.0  60.0
$coord frac
    0.00000000000000      0.00000000000000      0.00000000000000  ag
    0.50000000000000      0.50000000000000      0.50000000000000  br
$end

2c-SVWN (V)
$cell  angs
    3.9626048018     3.9626048018     3.9626048018    60.0       60.0      60.0
$coord frac
    0.00000000000000      0.00000000000000      0.00000000000000  ag
    0.50000000000000      0.50000000000000      0.50000000000000  br
$end

2c-PBE
$cell  angs
   4.13617434303333333333   4.13617434303333333333   4.13617434303333333333  60.0  60.0  60.0
$coord frac
    0.00000000000000      0.00000000000000      0.00000000000000  ag
    0.50000000000000      0.50000000000000      0.50000000000000  br
$end

2c-PBEsol
$cell  angs
   4.02480791976666666666   4.02480791976666666666   4.02480791976666666666   60.0   60.0   60.0
$coord frac
    0.00000000000000      0.00000000000000      0.00000000000000  ag
    0.50000000000000      0.50000000000000      0.50000000000000  br
$end
```

```
2c-TPSS
$cell  angs
   4.11004402016666666666   4.11004402016666666666   4.11004402016666666666   60.0   60.0   60.0
$coord frac
    0.00000000000000      0.00000000000000      0.00000000000000  ag
    0.50000000000000      0.50000000000000      0.50000000000000  br
$end

2c-revTPSS
$cell  angs
   4.0897251878   4.0897251878  4.0897251878   60.0  60.0  60.0
$coord frac
    0.00000000000000      0.00000000000000      0.00000000000000  ag
    0.50000000000000      0.50000000000000      0.50000000000000  br
$end

2c-Tao-Mo
$cell  angs
   4.05717500276666666666   4.05717500276666666666   4.05717500276666666666   60.0   60.0   60.0
$coord frac
    0.00000000000000      0.00000000000000      0.00000000000000  ag
    0.50000000000000      0.50000000000000      0.50000000000000  br
$end

2c-PKZB
$cell  angs
   4.14933946790000000000   4.14933946790000000000   4.14933946790000000000   60.0   60.0   60.0
$coord frac
    0.00000000000000      0.00000000000000      0.00000000000000  ag
    0.50000000000000      0.50000000000000      0.50000000000000  br
$end

2c-r2SCAN
$cell  angs
   4.10922457123333333333   4.10922457123333333333   4.10922457123333333333   60.0   60.0   60.0
$coord frac
    0.00000000000000      0.00000000000000      0.00000000000000  ag
    0.50000000000000      0.50000000000000      0.50000000000000  br
$end
```

iii) AgI

SVWN (V)

```
$cell  angs
  4.19916806426666666666   4.19916806426666666666  4.19916806426666666666  60.0  60.0   60.0
$coord frac
    0.00000000000000      0.00000000000000      0.00000000000000  ag
    0.50000000000000      0.50000000000000      0.50000000000000  i
$end
```

PBE

```
$cell  angs
  4.375962455  4.375962455  4.375962455  60.0  60.0  60.0
$coord frac
    0.00000000000000      0.00000000000000      0.00000000000000  ag
    0.50000000000000      0.50000000000000      0.50000000000000  i
$end
```

PBEsol

```
$cell  angs
  4.2604273368  4.2604273368  4.2604273368  60.0  60.0  60.0
$coord frac
    0.00000000000000      0.00000000000000      0.00000000000000  ag
    0.50000000000000      0.50000000000000      0.50000000000000  i
$end
```

TPSS

```
$cell  angs
  4.35287278606666666666  4.35287278606666666666  4.35287278606666666666  60.0   60.0  60.0
$coord frac
    0.00000000000000      0.00000000000000      0.00000000000000  ag
    0.50000000000000      0.50000000000000      0.50000000000000  i
$end
```

revTPSS

```
$cell  angs
   4.326282372  4.326282372   4.326282372  60.0   60.0   60.0
$coord frac
    0.00000000000000      0.00000000000000      0.00000000000000  ag
    0.50000000000000      0.50000000000000      0.50000000000000  i
$end
```

```
Tao-Mo
$cell  angs
   4.31120483906666666666  4.31120483906666666666  4.31120483906666666666   60.0   60.0  60.0
$coord frac
    0.00000000000000      0.00000000000000      0.00000000000000  ag
    0.50000000000000      0.50000000000000      0.50000000000000  i
$end

PKZB
$cell  angs
   4.38623378086666666666  4.38623378086666666666  4.38623378086666666666  60.0  60.0  60.0
$coord frac
    0.00000000000000      0.00000000000000      0.00000000000000  ag
    0.50000000000000      0.50000000000000      0.50000000000000  i
$end

r2SCAN
$cell  angs
  4.35615418616666666666  4.35615418616666666666  4.35615418616666666666  60.0  60.0  60.0
$coord frac
    0.00000000000000      0.00000000000000      0.00000000000000  ag
    0.50000000000000      0.50000000000000      0.50000000000000  i
$end

2c-SVWN (V)
$cell  angs
   4.19790823766666666666   4.19790823766666666666   4.19790823766666666666  60.0 60.0 60.0
$coord frac
    0.00000000000000      0.00000000000000      0.00000000000000  ag
    0.50000000000000      0.50000000000000      0.50000000000000  i
$end

2c-PBE
$cell  angs
   4.374539102   4.374539102   4.374539102   60.0   60.0   60.0
$coord frac
    0.00000000000000      0.00000000000000      0.00000000000000  ag
    0.50000000000000      0.50000000000000      0.50000000000000  i
$end

2c-PBEsol
$cell  angs
   4.25857171496666666666   4.25857171496666666666   4.25857171496666666666   60.0   60.0   60.0
$coord frac
    0.00000000000000      0.00000000000000      0.00000000000000  ag
    0.50000000000000      0.50000000000000      0.50000000000000  i
$end
```

```
2c-TPSS
$cell  angs
   4.35102446196666666666   4.35102446196666666666   4.35102446196666666666  60.0   60.0   60.0
$coord frac
    0.00000000000000      0.00000000000000      0.00000000000000  ag
    0.50000000000000      0.50000000000000      0.50000000000000  i
$end

2c-revTPSS
$cell  angs
  4.32457321323333333333  4.32457321323333333333  4.32457321323333333333  60.0   60.0   60.0
$coord frac
    0.00000000000000      0.00000000000000      0.00000000000000  ag
    0.50000000000000      0.50000000000000      0.50000000000000  i
$end

2c-Tao-Mo
$cell  angs
   4.2926534394   4.2926534394   4.2926534394  60.0   60.0   60.0
$coord frac
    0.00000000000000      0.00000000000000      0.00000000000000  ag
    0.50000000000000      0.50000000000000      0.50000000000000  i
$end

2c-PKZB
$cell  angs
   4.38391013183333333333   4.38391013183333333333   4.38391013183333333333   60.0   60.0   60.0
$coord frac
    0.00000000000000      0.00000000000000      0.00000000000000  ag
    0.50000000000000      0.50000000000000      0.50000000000000  i
$end

2c-r2SCAN
$cell  angs
   4.35527771656666666666   4.35527771656666666666   4.35527771656666666666   60.0    60.0   60.0
$coord frac
    0.00000000000000      0.00000000000000      0.00000000000000  ag
    0.50000000000000      0.50000000000000      0.50000000000000  i
$end
```

c) Relaxed structures with D3-BJ

i) AgCl

PBE-D3-BJ

```
$cell  angs
  3.92879622146666666666  3.92879622146666666666  3.92879622146666666666  60.0  60.0 60.0
$coord frac
    0.00000000000000      0.00000000000000      0.00000000000000  ag
    0.50000000000000      0.50000000000000      0.50000000000000  cl
$end
```

PBEsol-D3-BJ

```
$cell  angs
  3.83841735613333333333  3.83841735613333333333  3.83841735613333333333  60.0 60.0 60.0
$coord frac
    0.00000000000000      0.00000000000000      0.00000000000000  ag
    0.50000000000000      0.50000000000000      0.50000000000000  cl
$end
```

TPSS-D3-BJ

```
$cell  angs
  3.88912460836666666666  3.88912460836666666666  3.88912460836666666666  60.0 60.0 60.0
$coord frac
    0.00000000000000      0.00000000000000      0.00000000000000  ag
    0.50000000000000      0.50000000000000      0.50000000000000  cl
$end
```

revTPSS-D3-BJ

```
$cell  angs
  3.87246070486666666666  3.87246070486666666666  3.87246070486666666666  60.0  60.0  60.0
$coord frac
    0.00000000000000      0.00000000000000      0.00000000000000  ag
    0.50000000000000      0.50000000000000      0.50000000000000  cl
$end
```

Tao-Mo-D3-BJ

```
$cell  angs
  3.8983235666  3.8983235666  3.8983235666  60.0   60.0   60.0
$coord frac
    0.00000000000000      0.00000000000000      0.00000000000000  ag
    0.50000000000000      0.50000000000000      0.50000000000000  cl
$end
```

```
r2SCAN-D3-BJ
$cell  angs
  3.913670709  3.913670709  3.913670709  60.0   60.0   60.0
$coord frac
    0.00000000000000      0.00000000000000      0.00000000000000  ag
    0.50000000000000      0.50000000000000      0.50000000000000  cl
$end

2c-PBE-D3-BJ
$cell  angs
  3.91521636993333333333  3.91521636993333333333  3.91521636993333333333  60.0  60.0  60.0
$coord frac
    0.00000000000000      0.00000000000000      0.00000000000000  ag
    0.50000000000000      0.50000000000000      0.50000000000000  cl
$end

2c-PBEsol-D3-BJ
$cell  angs
  3.83689838036666666666  3.83689838036666666666  3.83689838036666666666  60.0  60.0  60.0
$coord frac
    0.00000000000000      0.00000000000000      0.00000000000000  ag
    0.50000000000000      0.50000000000000      0.50000000000000  cl
$end

2c-TPSS-D3-BJ
$cell  angs
  3.8874918142  3.8874918142  3.8874918142  60.0  60.0  60.0
$coord frac
    0.00000000000000      0.00000000000000      0.00000000000000  ag
    0.50000000000000      0.50000000000000      0.50000000000000  cl
$end

2c-revTPSS-D3-BJ
$cell  angs
  3.8711454888  3.8711454888  3.8711454888  60.0  60.0  60.0
$coord frac
    0.00000000000000      0.00000000000000      0.00000000000000  ag
    0.50000000000000      0.50000000000000      0.50000000000000  cl
$end

2c-Tao-Mo-D3-BJ
$cell  angs
  3.8970339839  3.8970339839  3.8970339839  60.0  60.0  60.0
$coord frac
    0.00000000000000      0.00000000000000      0.00000000000000  ag
    0.50000000000000      0.50000000000000      0.50000000000000  cl
$end
```

```
2c-r2SCAN-D3-BJ
$cell  angs
  3.90136349976666666666  3.90136349976666666666  3.90136349976666666666  60.0  60.0  60.0
$coord frac
    0.00000000000000      0.00000000000000      0.00000000000000  ag
    0.50000000000000      0.50000000000000      0.50000000000000  cl
$end
```

ii) AgBr

```
PBE-D3-BJ
$cell  angs
  4.0656560669  4.0656560669  4.0656560669  60.0  60.0  60.0
$coord frac
    0.00000000000000      0.00000000000000      0.00000000000000  ag
    0.50000000000000      0.50000000000000      0.50000000000000  br
$end

PBEsol-D3-BJ
$cell  angs
  3.9711451685  3.9711451685  3.9711451685  60.0  60.0  60.0
$coord frac
    0.00000000000000      0.00000000000000      0.00000000000000  ag
    0.50000000000000      0.50000000000000      0.50000000000000  br
$end

TPSS-D3-BJ
$cell  angs
  4.0377456864  4.0377456864  4.0377456864  60.0  60.0  60.0
$coord frac
    0.00000000000000      0.00000000000000      0.00000000000000  ag
    0.50000000000000      0.50000000000000      0.50000000000000  br
$end

revTPSS-D3-BJ
$cell  angs
  4.02469085823333333333  4.02469085823333333333  4.02469085823333333333  60.0   60.0  60.0
$coord frac
    0.00000000000000      0.00000000000000      0.00000000000000  ag
    0.50000000000000      0.50000000000000      0.50000000000000  br
$end

Tao-Mo-D3-BJ
$cell  angs
  4.06252851366666666666  4.06252851366666666666  4.06252851366666666666  60.0  60.0  60.0
$coord frac
    0.00000000000000      0.00000000000000      0.00000000000000  ag
    0.50000000000000      0.50000000000000      0.50000000000000  br
$end
```

```
r2SCAN-D3-BJ
$cell  angs
  4.082712298  4.082712298  4.082712298  60.0  60.0  60.0
$coord frac
    0.00000000000000      0.00000000000000      0.00000000000000  ag
    0.50000000000000      0.50000000000000      0.50000000000000  br
$end

2c-PBE-D3-BJ
$cell  angs
  4.06356866316666666666  4.06356866316666666666  4.06356866316666666666  60.0  60.0  60.0
$coord frac
    0.00000000000000      0.00000000000000      0.00000000000000  ag
    0.50000000000000      0.50000000000000      0.50000000000000  br
$end

2c-PBEsol-D3-BJ
$cell  angs
  3.96911415466666666666  3.96911415466666666666  3.96911415466666666666  60.0  60.0  60.0
$coord frac
    0.00000000000000      0.00000000000000      0.00000000000000  ag
    0.50000000000000      0.50000000000000      0.50000000000000  br
$end

2c-TPSS-D3-BJ
$cell  angs
  4.03638224546666666666  4.03638224546666666666  4.03638224546666666666  60.0  60.0  60.0
$coord frac
    0.00000000000000      0.00000000000000      0.00000000000000  ag
    0.50000000000000      0.50000000000000      0.50000000000000  br
$end

2c-revTPSS-D3-BJ
$cell  angs
  4.0234614894  4.0234614894  4.0234614894  60.0  60.0  60.0
$coord frac
    0.00000000000000      0.00000000000000      0.00000000000000  ag
    0.50000000000000      0.50000000000000      0.50000000000000  br
$end

2c-Tao-Mo-D3-BJ
$cell  angs
  4.0611942705  4.0611942705  4.0611942705  60.0  60.0  60.0
$coord frac
    0.00000000000000      0.00000000000000      0.00000000000000  ag
    0.50000000000000      0.50000000000000      0.50000000000000  br
$end
```

```
2c-r2SCAN-D3-BJ
$cell  angs
  4.0811353733  4.0811353733  4.0811353733  60.0  60.0  60.0
$coord frac
    0.00000000000000      0.00000000000000      0.00000000000000  ag
    0.50000000000000      0.50000000000000      0.50000000000000  br
$end
```

iii) AgI

PBE-D3-BJ

```
$cell  angs
  4.29762263753333333333  4.29762263753333333333  4.29762263753333333333  60.0  60.0  60.0
$coord frac
    0.00000000000000      0.00000000000000      0.00000000000000  ag
    0.50000000000000      0.50000000000000      0.50000000000000  i
$end
```

PBEsol-D3-BJ

```
$cell  angs
  4.19283430466666666666  4.19283430466666666666  4.19283430466666666666  60.0  60.0  60.0
$coord frac
    0.00000000000000      0.00000000000000      0.00000000000000  ag
    0.50000000000000      0.50000000000000      0.50000000000000  i
$end
```

TPSS-D3-BJ

```
$cell  angs
  4.23056622496666666666  4.23056622496666666666  4.23056622496666666666   60.0   60.0  60.0
$coord frac
    0.00000000000000      0.00000000000000      0.00000000000000  ag
    0.50000000000000      0.50000000000000      0.50000000000000  i
$end
```

revTPSS-D3-BJ

```
$cell  angs
  4.2109555586 4.2109555586 4.2109555586 60.0 60.0  60.0
$coord frac
    0.00000000000000      0.00000000000000      0.00000000000000  ag
    0.50000000000000      0.50000000000000      0.50000000000000  i
$end
```

Tao-Mo-D3-BJ

```
$cell  angs
  4.29789857256666666666  4.29789857256666666666  4.29789857256666666666  60.0  60.0  60.0
$coord frac
    0.00000000000000      0.00000000000000      0.00000000000000  ag
    0.50000000000000      0.50000000000000      0.50000000000000  i
$end
```

```
r2SCAN-D3-BJ
$cell  angs
  4.3548993639  4.3548993639  4.3548993639  60.0  60.0 60.0
$coord frac
    0.00000000000000      0.00000000000000      0.00000000000000  ag
    0.50000000000000      0.50000000000000      0.50000000000000  i
$end

2c-PBE-D3-BJ
$cell  angs
  4.2899779228  4.2899779228  4.2899779228  60.0  60.0  60.0
$coord frac
    0.00000000000000      0.00000000000000      0.00000000000000  ag
    0.50000000000000      0.50000000000000      0.50000000000000  i
$end

2c-PBEsol-D3-BJ
$cell  angs
  4.19121877706666666666  4.19121877706666666666  4.19121877706666666666  60.0  60.0  60.0
$coord frac
    0.00000000000000      0.00000000000000      0.00000000000000  ag
    0.50000000000000      0.50000000000000      0.50000000000000  i
$end

2c-TPSS-D3-BJ
$cell  angs
  4.22982934023333333333  4.22982934023333333333 4.22982934023333333333  60.0  60.0  60.0
$coord frac
    0.00000000000000      0.00000000000000      0.00000000000000  ag
    0.50000000000000      0.50000000000000      0.50000000000000  i
$end

2c-revTPSS-D3-BJ
$cell  angs
  4.20627833826666666666  4.20627833826666666666  4.20627833826666666666  60.0  60.0  60.0
$coord frac
    0.00000000000000      0.00000000000000      0.00000000000000  ag
    0.50000000000000      0.50000000000000      0.50000000000000  i
$end

2c-Tao-Mo-D3-BJ
$cell  angs
  4.29099278693333333333  4.29099278693333333333  4.29099278693333333333  60.0  60.0  60.0
$coord frac
    0.00000000000000      0.00000000000000      0.00000000000000  ag
    0.50000000000000      0.50000000000000      0.50000000000000  i
$end
```

```
2c-r2SCAN-D3-BJ
$cell  angs
  4.3530927047  4.3530927047  4.3530927047  60.0  60.0  60.0
$coord frac
    0.00000000000000      0.00000000000000      0.00000000000000  ag
    0.50000000000000      0.50000000000000      0.50000000000000  i
$end
```

## E. Indium(I,III)-Telluride Two-Dimensional Honeycomb System

a) 1c optimization without D3

```
$cell
 8.0124390 8.0124390 60.0
$coord
    0.00000000000000      0.00000000000000      0.00000000000000      in
    0.00125810178926      0.00074629401429      5.30945552703617      in
    4.00628439107714      2.31300606929462     -2.75618224113402      te
    4.00743098931212      2.31368907685671      8.06634157724272      te
$end
```

b) 1c optimization with D3

```
$cell
  8.1284346 8.1284346 60.0
$coord
    0.00000000000000      0.00000000000000      0.00000000000000  in
    0.00000000000000      0.00000000000000      5.26273509093640  in
    4.05997252052396      2.34549030506129     -2.67054225966576  te
    4.05997252052396      2.34549030506129      7.93471996528309  te
$end
```

c) 2c optimization with D3

```
$cell
  8.1284346 8.1284346 60.0
$coord
    0.00000000000000      0.00000000000000      0.00000000000000  in
    0.00000000000000      0.00000000000000      5.26273509093640  in
    4.05997252052396      2.34549030506129     -2.67054225966576  te
    4.05997252052396      2.34549030506129      7.93471996528309  te
$end
```

## F. One-Dimensional Platinum Chains

```
$cell angs
4.0
$coord
    0.00000000000000     0.00000000000000     0.00000000000000     pt
    3.77945197720000     0.00000000000000     0.00000000000000     pt
$end

$cell angs
4.1
$coord
    0.00000000000000     0.00000000000000     0.00000000000000     pt
    3.87393827660000     0.00000000000000     0.00000000000000     pt
$end

$cell angs
4.2
$coord
    0.00000000000000     0.00000000000000     0.00000000000000     pt
    3.96842457600000     0.00000000000000     0.00000000000000     pt
$end

$cell angs
4.3
$coord
    0.00000000000000     0.00000000000000     0.00000000000000     pt
    4.06291087540000     0.00000000000000     0.00000000000000     pt
$end

$cell angs
4.4
$coord
    0.00000000000000     0.00000000000000     0.00000000000000     pt
    4.15739717490000     0.00000000000000     0.00000000000000     pt
$end

$cell angs
4.5
$coord
    0.00000000000000     0.00000000000000     0.00000000000000     pt
    4.25188347430000     0.00000000000000     0.00000000000000     pt
$end
```

```
$cell angs
4.6
$coord
    0.00000000000000     0.00000000000000     0.00000000000000     pt
    4.34636977370000     0.00000000000000     0.00000000000000     pt
$end

$cell angs
4.7
$coord
    0.00000000000000     0.00000000000000     0.00000000000000     pt
    4.44085607320000     0.00000000000000     0.00000000000000     pt
$end

$cell angs
4.8
$coord
    0.00000000000000     0.00000000000000     0.00000000000000     pt
    4.53534237260000     0.00000000000000     0.00000000000000     pt
$end

$cell angs
4.9
$coord
    0.00000000000000     0.00000000000000     0.00000000000000     pt
    4.62982867200000     0.00000000000000     0.00000000000000     pt
$end

$cell angs
5.0
$coord
    0.00000000000000     0.00000000000000     0.00000000000000     pt
    4.72431497140000     0.00000000000000     0.00000000000000     pt
$end

$cell ang
5.02
$coord
    0.00000000000000     0.00000000000000     0.00000000000000     pt
    4.74321300000000     0.00000000000000     0.00000000000000     pt
$end

$cell ang
5.04
$coord
    0.00000000000000     0.00000000000000     0.00000000000000     pt
    4.76211000000000     0.00000000000000     0.00000000000000     pt
$end
```

```
$cell ang
5.06
$coord
    0.00000000000000      0.00000000000000      0.00000000000000      pt
    4.78100700000000      0.00000000000000      0.00000000000000      pt
$end

$cell ang
5.08
$coord
    0.00000000000000      0.00000000000000      0.00000000000000      pt
    4.79990400000000      0.00000000000000      0.00000000000000      pt

$cell angs
5.1
$coord
    0.00000000000000      0.00000000000000      0.00000000000000      pt
    4.81880127090000      0.00000000000000      0.00000000000000      pt
$end

$cell angs
5.15
$coord
    0.00000000000000      0.00000000000000      0.00000000000000      pt
    4.86604500000000      0.00000000000000      0.00000000000000      pt
$end

$cell angs
5.2
$coord
    0.00000000000000      0.00000000000000      0.00000000000000      pt
    4.91328757030000      0.00000000000000      0.00000000000000      pt
$end

$cell angs
5.25
$coord
    0.00000000000000      0.00000000000000      0.00000000000000      pt
    4.96053100000000      0.00000000000000      0.00000000000000      pt
$end

$cell angs
5.3
$coord
    0.00000000000000      0.00000000000000      0.00000000000000      pt
    5.00777386970000      0.00000000000000      0.00000000000000      pt
$end
```

```
$cell angs
5.35
$coord
    0.00000000000000    0.00000000000000    0.00000000000000    pt
    5.05501500000000    0.00000000000000    0.00000000000000    pt
$end

$cell angs
5.4
$coord
    0.00000000000000    0.00000000000000    0.00000000000000    pt
    5.10226016920000    0.00000000000000    0.00000000000000    pt
$end

$cell angs
5.5
$coord
    0.00000000000000    0.00000000000000    0.00000000000000    pt
    5.19674646860000    0.00000000000000    0.00000000000000    pt
$end

$cell angs
5.6
$coord
    0.00000000000000    0.00000000000000    0.00000000000000    pt
    5.29123276800000    0.00000000000000    0.00000000000000    pt
$end

$cell angs
5.7
$coord
    0.00000000000000    0.00000000000000    0.00000000000000    pt
    5.38571906740000    0.00000000000000    0.00000000000000    pt
$end

$cell angs
5.8
$coord
    0.00000000000000    0.00000000000000    0.00000000000000    pt
    5.48020536690000    0.00000000000000    0.00000000000000    pt
$end
```

```
$cell angs
5.9
$coord
    0.00000000000000      0.00000000000000      0.00000000000000      pt
    5.57469166630000      0.00000000000000      0.00000000000000      pt
$end

$cell angs
6.0
$coord
    0.00000000000000      0.00000000000000      0.00000000000000      pt
    5.66917796570000      0.00000000000000      0.00000000000000      pt
$end
```

[1] R. Zhao, Y. Zhang, Y. Xiao, and W. Liu, Exact two-component relativistic energy band theory and application, J. Chem. Phys. **144**, 044105 (2016).

[2] J. C. Slater, A simplification of the Hartree–Fock method, Phys. Rev. **81**, 385 (1951).

[3] S. H. Vosko, L. Wilk, and M. Nusair, Accurate spin-dependent electron liquid correlation energies for local spin density calculations: a critical analysis, Can. J. Phys. **58**, 1200 (1980).

[4] J. P. Perdew, K. Burke, and M. Ernzerhof, Generalized gradient approximation made simple, Phys. Rev. Lett. **77**, 3865 (1996).

[5] J. P. Perdew, A. Ruzsinszky, G. I. Csonka, O. A. Vydrov, G. E. Scuseria, L. A. Constantin, X. Zhou, and K. Burke, Restoring the density-gradient expansion for exchange in solids and surfaces, Phys. Rev. Lett. **100**, 136406 (2008).

[6] J. Tao, J. P. Perdew, V. N. Staroverov, and G. E. Scuseria, Climbing the density functional ladder: Nonempirical meta–generalized gradient approximation designed for molecules and solids, Phys. Rev. Lett. **91**, 146401 (2003).

[7] J. P. Perdew, A. Ruzsinszky, G. I. Csonka, L. A. Constantin, and J. Sun, Workhorse semilocal density functional for condensed matter physics and quantum chemistry, Phys. Rev. Lett. **103**, 026403 (2009).

[8] J. P. Perdew, A. Ruzsinszky, G. I. Csonka, L. A. Constantin, and J. Sun, Erratum: Workhorse semilocal density functional for condensed matter physics and quantum chemistry [Phys. Rev. Lett. 103, 026403 (2009)], Phys. Rev. Lett. **106**, 179902(E) (2011).

[9] J. Tao and Y. Mo, Accurate semilocal density functional for condensed-matter physics and quantum chemistry, Phys. Rev. Lett. **117**, 073001 (2016).

[10] J. P. Perdew, S. Kurth, A. Zupan, and P. Blaha, Accurate density functional with correct formal properties: A step beyond the generalized gradient approximation, Phys. Rev. Lett. **82**, 2544 (1999).

[11] J. W. Furness, A. D. Kaplan, J. Ning, J. P. Perdew, and J. Sun, Accurate and numerically efficient r$^2$SCAN meta-generalized gradient approximation, J. Phys. Chem. Lett. **11**, 8208 (2020).

[12] J. W. Furness, A. D. Kaplan, J. Ning, J. P. Perdew, and J. Sun, Correction to "Accurate and numerically efficient r$^2$SCAN meta-generalized gradient approximation", J. Phys. Chem. Lett. **11**, 9248 (2020).

[13] M. A. L. Marques, M. J. T. Oliveira, and T. Burnus, Libxc: A library of exchange and correlation functionals for density functional theory, Comput. Phys. Commun. **183**, 2272 (2012).

[14] S. Lehtola, C. Steigemann, M. J. T. Oliveira, and M. A. L. Marques, Recent developments in Libxc – a comprehensive library of functionals for density functional theory, SoftwareX **7**, 1 (2018).

[15] Libxc, Version 6.0.0, available from `https://www.tddft.org/programs/libxc/` (retrieved August 16, 2022).

[16] F. Weigend and A. Baldes, Segmented contracted basis sets for one- and two-component Dirac–Fock effective core potentials, J. Chem. Phys. **133**, 174102 (2010).

[17] S. Grimme, J. Antony, S. Ehrlich, and H. Krieg, A consistent and accurate *ab initio* parametrization of density functional dispersion correction (DFT-D) for the 94 elements H-Pu, J. Chem. Phys. **132**, 154104 (2010).

[18] S. Grimme, S. Ehrlich, and L. Goerigk, Effect of the damping function in dispersion corrected density functional theory, J. Comput. Chem. **32**, 1456 (2011).

[19] C. R. Berry, Physical defects in silver halides, Phys. Rev. **97**, 676 (1955).

[20] P. Wang, B. Huang, X. Zhang, X. Qin, H. Jin, Y. Dai, Z. Wang, J. Wei, J. Zhan, S. Wang, J. Wang, and M.-H. Whangbo, Highly efficient visible-light plasmonic photocatalyst Ag@AgBr, Chem. Eur. J. **15**, 1821 (2009).

[21] G. Piermarini and C. Weir, A diamond cell for X-ray diffraction studies at high pressures, J. Res. Natl. Bur. Stan., Sec. A **66**, 325 (1962).

[22] R. Łazarski, A. M. Burow, L. Grajciar, and M. Sierka, Density functional theory for molecular and periodic systems using density fitting and continuous fast multipole method: Analytical gradients, J. Comput. Chem. **37**, 2518 (2016).

[23] M. Becker and M. Sierka, Density functional theory for molecular and periodic systems using density fitting and continuous fast multipole method: Stress tensor, J. Comput. Chem. **40**, 2563 (2019).

[24] G. Kresse and J. Furthmüller, Efficiency of ab-initio total energy calculations for metals and semiconductors using a plane-wave basis set, Comput. Mater. Sci. **6**, 15 (1996).

[25] D. Figgen, K. A. Peterson, M. Dolg, and H. Stoll, Energy-consistent pseudopotentials and correlation consistent basis sets for the $5d$ elements Hf–Pt, J. Chem. Phys. **130**, 164108 (2009).

[26] J. Heyd, G. E. Scuseria, and M. Ernzerhof, Hybrid functionals based on a screened Coulomb potential, J. Chem. Phys. **118**, 8207 (2003).

[27] J. Heyd, G. E. Scuseria, and M. Ernzerhof, Erratum: "Hybrid functionals based on a screened Coulomb potential" [J. Chem. Phys. 118, 8207 (2003)], J. Phys. Chem. **124**, 219906 (2006).

[28] A. V. Krukau, O. A. Vydrov, A. F. Izmaylov, and G. E. Scuseria, Influence of the exchange screening parameter on the performance of screened hybrid functionals, J. Phys. Chem. **125**, 224106 (2006).

[29] R. Ahlrichs, M. Bär, M. Häser, H. Horn, and C. Kölmel, Electronic structure calculations on workstation computers: The program system turbomole, Chem. Phys. Lett. **162**, 165 (1989).

[30] Developers' version of TURBOMOLE V7.7 (2022), a development of University of Karlsruhe and Forschungszentrum Karlsruhe GmbH, 1989-2007, TURBOMOLE GmbH, since 2007; available from `https://www.turbomole.org` (retrieved May 4, 2023).

[31] Manual of TURBOMOLE V7.7 (2022), a development of University of Karlsruhe and Forschungszentrum Karlsruhe GmbH, 1989-2007, TURBOMOLE GmbH, since 2007; available from `https://www.turbomole.org/turbomole/turbomole-documentation/` (retrieved May 4, 2023).

[32] Y. J. Franzke, C. Holzer, J. H. Andersen, T. Begušić, F. Bruder, S. Coriani, F. Della Sala, E. Fabiano, D. A. Fedotov, S. Fürst, S. Gillhuber, R. Grotjahn, M. Kaupp, M. Kehry, M. Krstić, F. Mack, S. Majumdar, B. D. Nguyen, S. M. Parker, F. Pauly, A. Pausch, E. Perlt, G. S. Phun, A. Rajabi, D. Rappoport, B. Samal, T. Schrader, M. Sharma, E. Tapavicza, R. S. Treß, V. Voora, A. Wodyński, J. M. Yu, B. Zerulla, F. Furche, C. Hättig, M. Sierka, D. P. Tew, and F. Weigend, TURBOMOLE: Today and Tomorrow, J. Chem. Theory Comput. **19**, 6859 (2023).
